# Supplementary material for: A sparse Bayesian hierarchical vector autoregressive model for microbial dynamics in a wastewater treatment plant
Source: arXiv:2107.00502 ancillary file (2021-07-01)
Supplement: Supplementary file 1 [file supplMat.pdf]

# Supplementary Materials for Hannaford et al. (2021)

Naomi E. Hannaford[1], Sarah E. Heaps[1,*], Tom M. W. Nye[1], Thomas P. Curtis[2], Ben Allen[1], Andrew Golightly[1], and Darren J. Wilkinson[1]

[1]School of Mathematics, Statistics and Physics, Newcastle University, Newcastle upon Tyne, United Kingdom

[2]School of Engineering, Newcastle University, Newcastle upon Tyne, United Kingdom

[*]Corresponding author: sarah.heaps@ncl.ac.uk

## 1 VAR(1) model as a linear approximation to a Lotka-Volterra model

In the main text, we use a VAR(1) model as a linear approximation to a Lotka-Volterra model. Here we show why this is the case. First consider a *stochastic* Lotka-Volterra model with two species, given by the Itô stochastic differential equations

$$\begin{aligned} dy_1(t) &= \tilde{\alpha} y_1(t) - \beta y_1(t) y_2(t) + \sigma_1 dw_1(t) \\ dy_2(t) &= -\tilde{\delta} y_2(t) + \gamma y_1(t) y_2(t) + \sigma_2 dw_2(t), \end{aligned} \tag{1}$$

where $\tilde{\alpha}, \beta, \gamma, \tilde{\delta} \geq 0$ and $\{w_1(t), t \geq 0\}$ and $\{w_2(t), t \geq 0\}$ are independent Wiener processes. Let $\boldsymbol{Y}_t = (Y_{t,1}, Y_{t,2})^T$ denote an appropriate discretisation of the time series of the two species with time step $\Delta t$ so that $t_N = t_0 + n\Delta t$ for some initial time $t_0$, where $t_N$ is the last time point in the time series. Without loss of generality, taking $\Delta t = 1$, the Euler-Maruyama approximation to the solution of the stochastic differential equation driving the Lotka-Volterra model is

$$\begin{aligned} Y_{t+1,1} &= \alpha Y_{t,1} - \beta Y_{t,1} Y_{t,2} + \epsilon_{t,1} \\ Y_{t+1,2} &= -\delta Y_{t,2} + \gamma Y_{t,1} Y_{t,2} + \epsilon_{t,2}, \end{aligned} \tag{2}$$

where $\alpha, \beta, \gamma, \delta \geq 0$, $\boldsymbol{\epsilon}_t = (\epsilon_{t,1}, \epsilon_{t,2})^T \sim \mathrm{N}_2(\mathbf{0}, \Sigma)$ and $\Sigma = \mathrm{diag}(\sigma_1^2, \sigma_2^2)$. Interactions between the two population sizes $y_{t,1}$ and $y_{t,2}$ arise due to the coupling of the underpinning differential equations. In the numerical solution in (2), the dependence of $\boldsymbol{Y}_{t+1}$ on $\boldsymbol{Y}_t$ is non-linear.

Now consider a zero-mean VAR(1) model for a discrete time series with two species $\{\boldsymbol{Y}_t : t = 0, 1, \ldots.\}$. This can be expressed as

$$\begin{aligned} Y_{t+1,1} &= \alpha Y_{t,1} - \beta Y_{t,2} + \epsilon_{t,1} \\ Y_{t+1,2} &= -\delta Y_{t,2} + \gamma Y_{t,1} + \epsilon_{t,2}, \end{aligned} \tag{3}$$

where $\alpha, \beta, \gamma, \delta \in \mathbb{R}$ but we could impose a positivity constraint and $\boldsymbol{\epsilon}_t \sim \mathrm{N}_2(\mathbf{0}, \Sigma)$ as above for (2). Here the dependence of $\boldsymbol{Y}_{t+1}$ on $\boldsymbol{Y}_t$ is linear by construction. However, (3) and (2) show that the VAR(1) and Lotka-Volterra models share a similar structure. Thus, we can regard the VAR(1) as a linear approximation to the non-linear numerical solution of the Lotka-Volterra system.

## 2 Exploratory analysis

### 2.1 Data description

Table 1 shows the number of different types for each taxonomic rank, excluding unknown taxonomic ranks.

| Taxonomic Rank | |
|---|---|
| Kingdom | 3 |
| Phylum | 42 |
| Class | 84 |
| Order | 132 |
| Family | 272 |
| Genus | 713 |

Table 1: Number of different types for each taxonomic rank, excluding `NA`s.

### 2.2 Missing data

Table 2 shows the proportions of missing data for each taxonomic rank in the taxonomy table. Table 3 shows the proportions of missing chemical and environmental data.

| Taxonomic Rank | Proportion |
|---|---|
| Kingdom | 0.0108 |
| Phylum | 0.0532 |
| Class | 0.1202 |
| Order | 0.2021 |
| Family | 0.3014 |
| Genus | 0.5409 |

Table 2: Proportions of missing data (to four d.p.) for each taxonomic rank in the taxonomy table.

| Covariate | Proportion | Covariate | Proportion |
|---|---|---|---|
| COD | 0.0661 | Ammonia | 0.0661 |
| Nitrate | 0.0039 | Nitrite | 0.0039 |
| Sulphate | 0.0039 | Phosphate | 0.0039 |
| Fluoride | 0.0039 | Chloride | 0.0039 |
| pH | 0.0039 | Temperature | 0.0039 |
| DO | 0.0039 | | |

Table 3: Proportions of missing data (4 d.p.) in chemical/environmental data. MLSS and MLVSS are not shown as they have no missing data.

### 2.3 OTUs

Figure 1 shows a time series plot of the total number of OTUs in the activated sludge (AS). This does not represent the true total number but rather the *sampling depths* over time, which are the total numbers of sequences collected in each sample. Figure 2 shows the time series plots of the 12 most abundant OTUs. As we discuss in Section 2.2 of the main text, we can see annual cycles in many of the OTUs. Figure 3 shows the time series plots of OTU 1 and *Trichococcus* on the $\log_{10}$ scale. The plots are very similar because OTU 1 represents the majority of *Trichococcus*. Figure 4 shows the stacked bar plot for the top 12 OTUs, where the seasonal behaviour can also be seen.

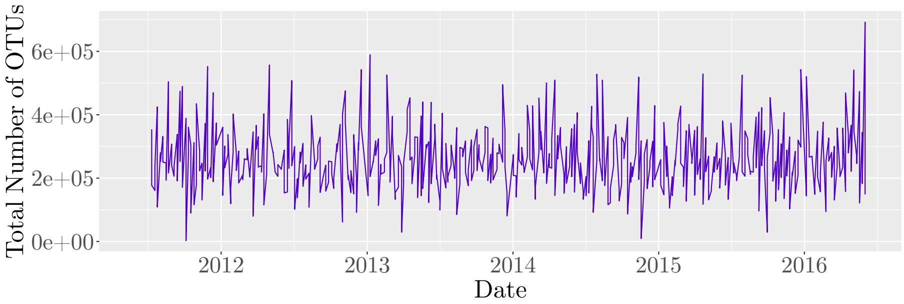


Figure 1: Time series plot of total abundance. Note that this does not represent the true total abundance but rather the sampling depths over time.

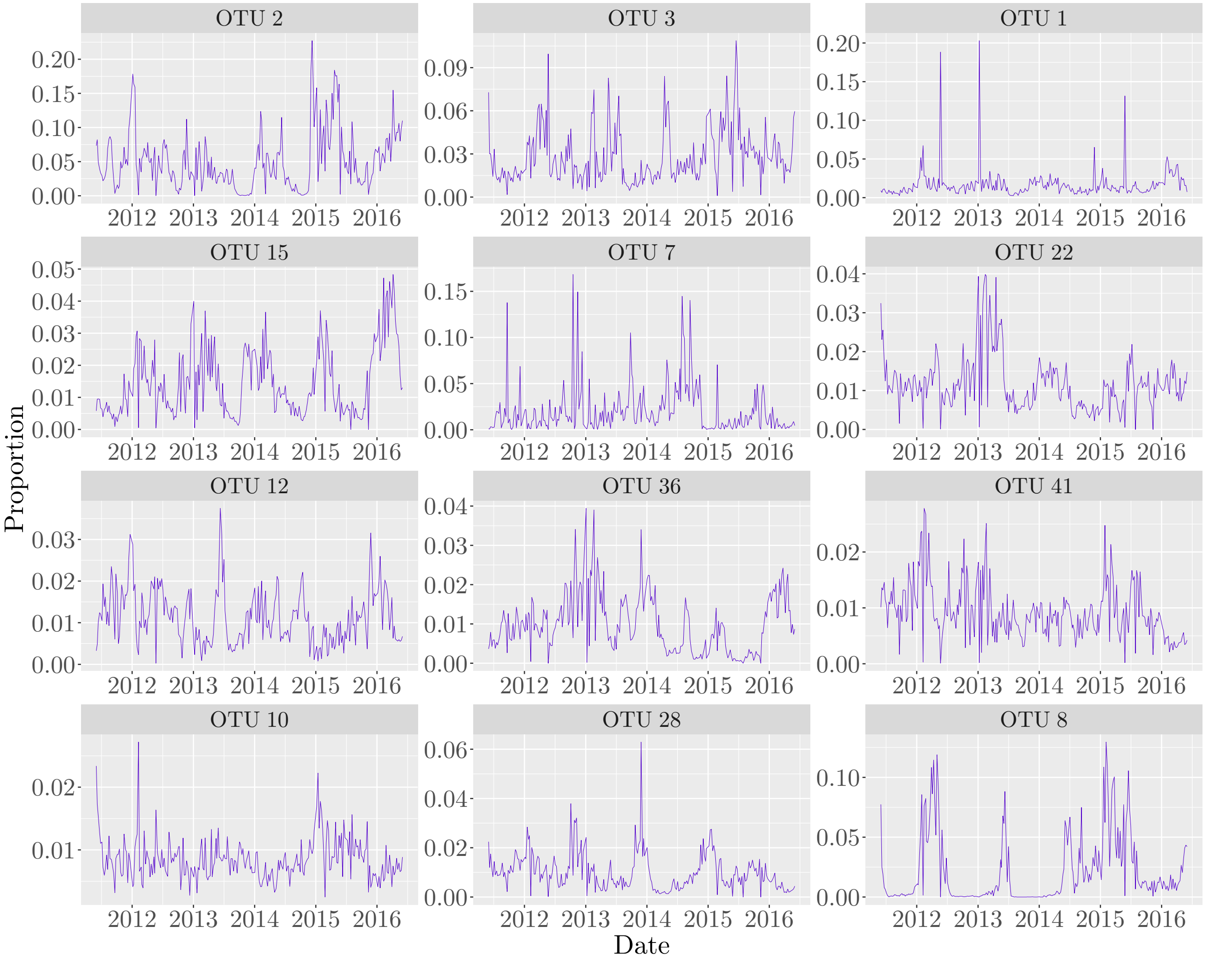


Figure 2: Time series plots for the top 12 OTUs based on median abundance.

## 2.4 Taxonomy

Figure 5 and Figure 7 show the time series plots of the top 12 genera and classes based on median abundance, respectively, which are discussed in Section 2.3 of the main text. Also discussed are Figures 6 and 8, which show their corresponding stacked bar plots.

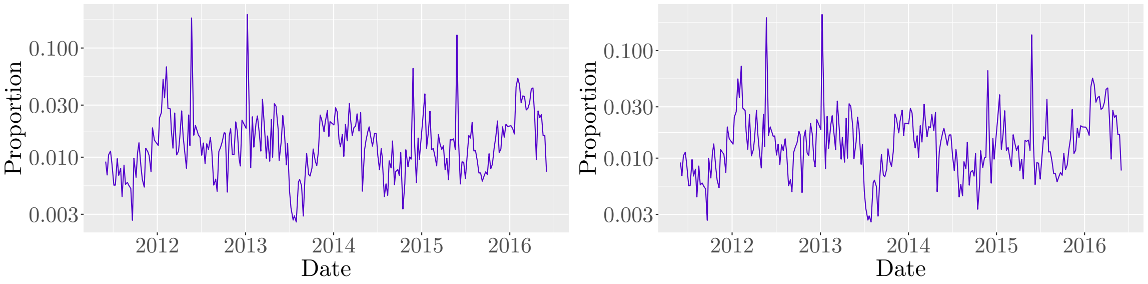


(a) (b)

Figure 3: Time series plot of (a) OTU 1 and (b) *Trichococcus* on $\log_{10}$ scale.

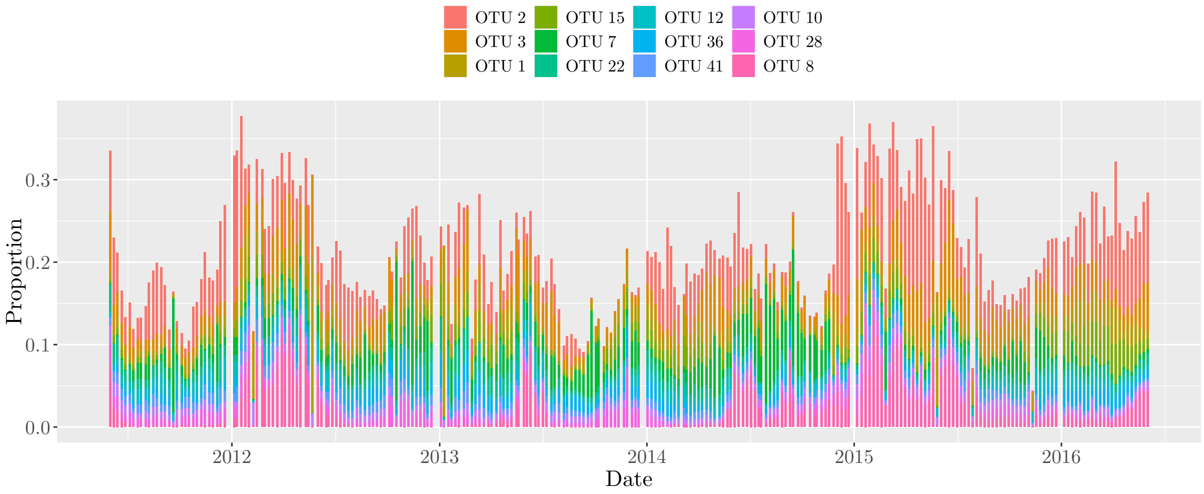


Figure 4: Stacked bar plot of the top 12 OTUs based on median abundance.

# 3 Reparameterisation of symmetric, circulant, tridiagonal precision matrix

A $(K \times K)$ symmetric, circulant, tridiagonal precision matrix is given in (3) in Section 4.1 of the main text. Its eigenvalues are $\eta_j = \sigma_0^{-2} + 2\omega \cos(2\pi j/K)$ for $j = 0, 1, \ldots, K-1$. It is positive definite if

$$\eta_j > 0 \Leftrightarrow \sigma_0^{-2} > -2\omega \cos(2\pi j/K) \qquad \text{for all } j.$$

Suppose that $\omega < 0$, then we require

$$-\sigma_0^{-2}/(2\omega) > \cos(2\pi j/K).$$

This is true if $-\sigma_0^{-2}/(2\omega) > 1$, which can only occur when $\sigma_0^{-2} > 0$. Now suppose $\omega > 0$. Then we require

$$-\sigma_0^{-2}/(2\omega) < \cos(2\pi j/K).$$

This is true if $-\sigma_0^{-2}/(2\omega) < -1$, i.e. $\sigma_0^{-2}/(2\omega) > 1$, which can only occur when $\sigma_0^{-2} > 0$. Altogether, this means we require $\sigma_0^{-2}/(2|\omega|) > 1$, i.e. $\sigma_0^{-2} > 2|\omega|$, whilst $\omega \in \mathbb{R}$. Parameterisations

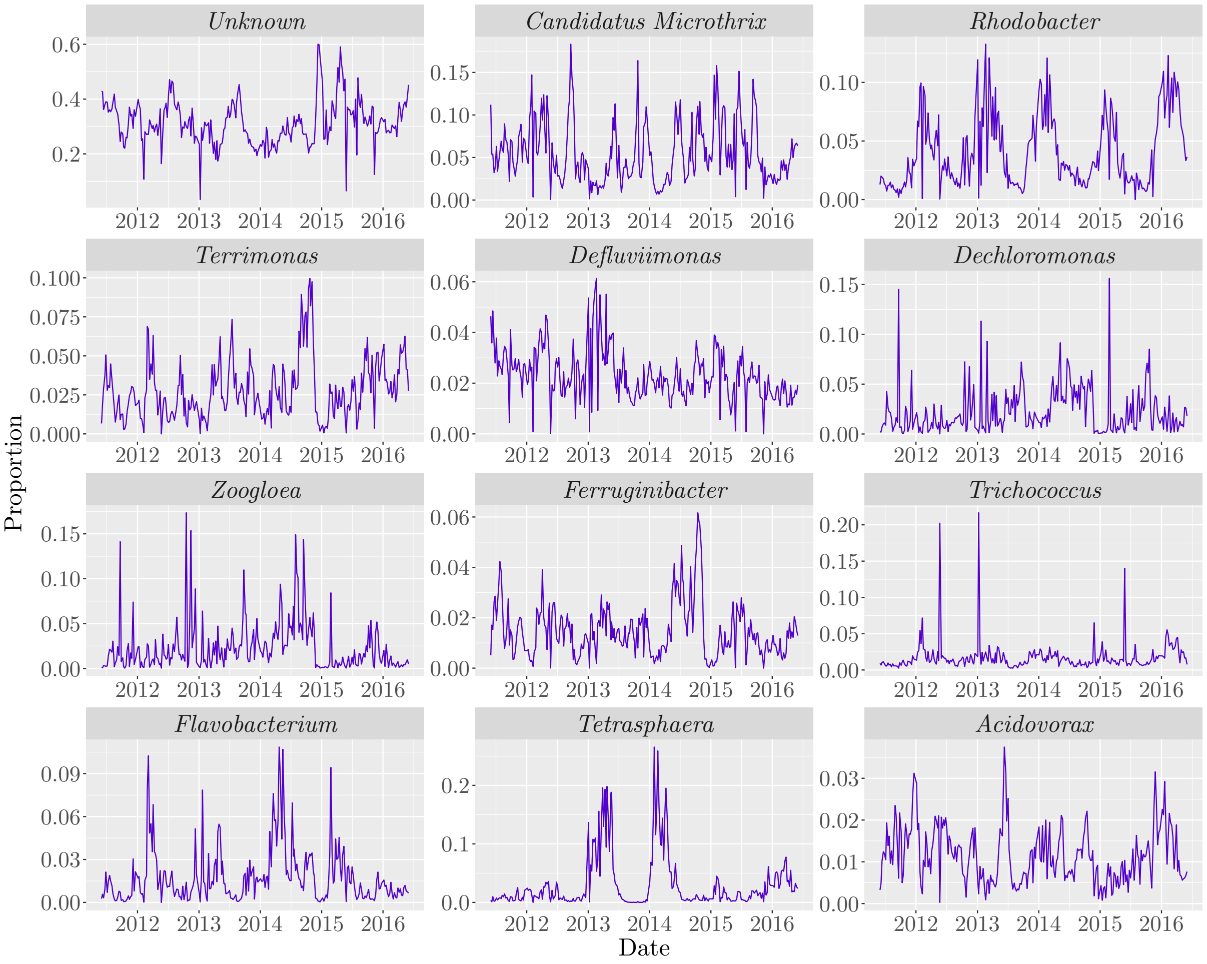


Figure 5: Time series plot for the top 12 genera based on median abundance.

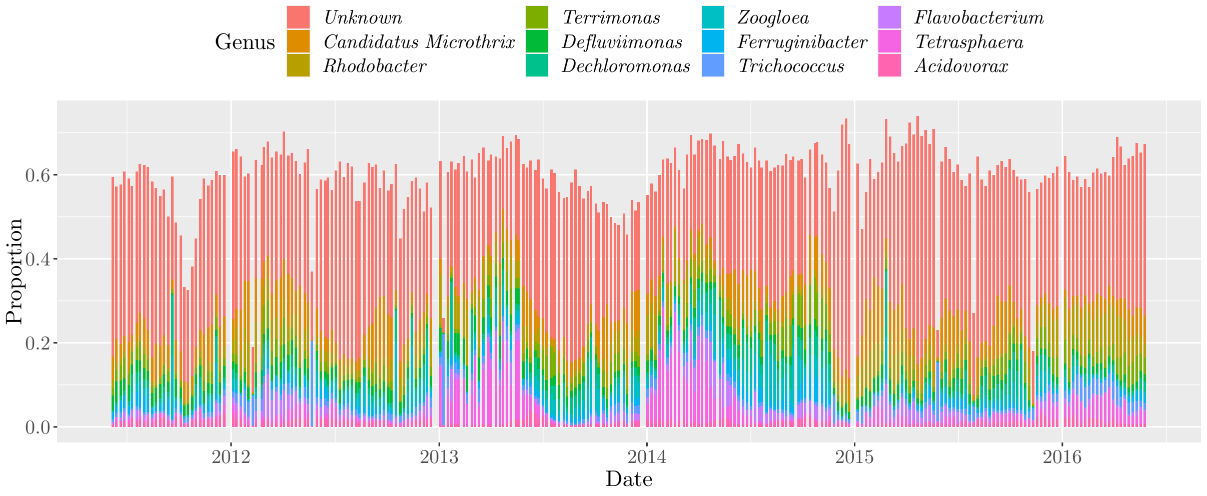


Figure 6: Stacked bar plot for the top 12 genera based on median abundance.

over fixed regions are generally nicer, so we parameterise in terms of $\bar{\omega}_0$ and $\bar{\omega}_1$, where

$$\begin{aligned} \sigma_0^{-2} &= \left(\varpi_0 + \varpi_1\right)/\sqrt{2} \\ \omega &= \left(\varpi_0 - \varpi_1\right)/2\sqrt{2} \\ \varpi_0 &= \sqrt{2}\left(\sigma_0^{-2} + 2\omega\right)/2 \\ \varpi_1 &= \sqrt{2}\left(\sigma_0^{-2} - 2\omega\right)/2, \end{aligned}$$

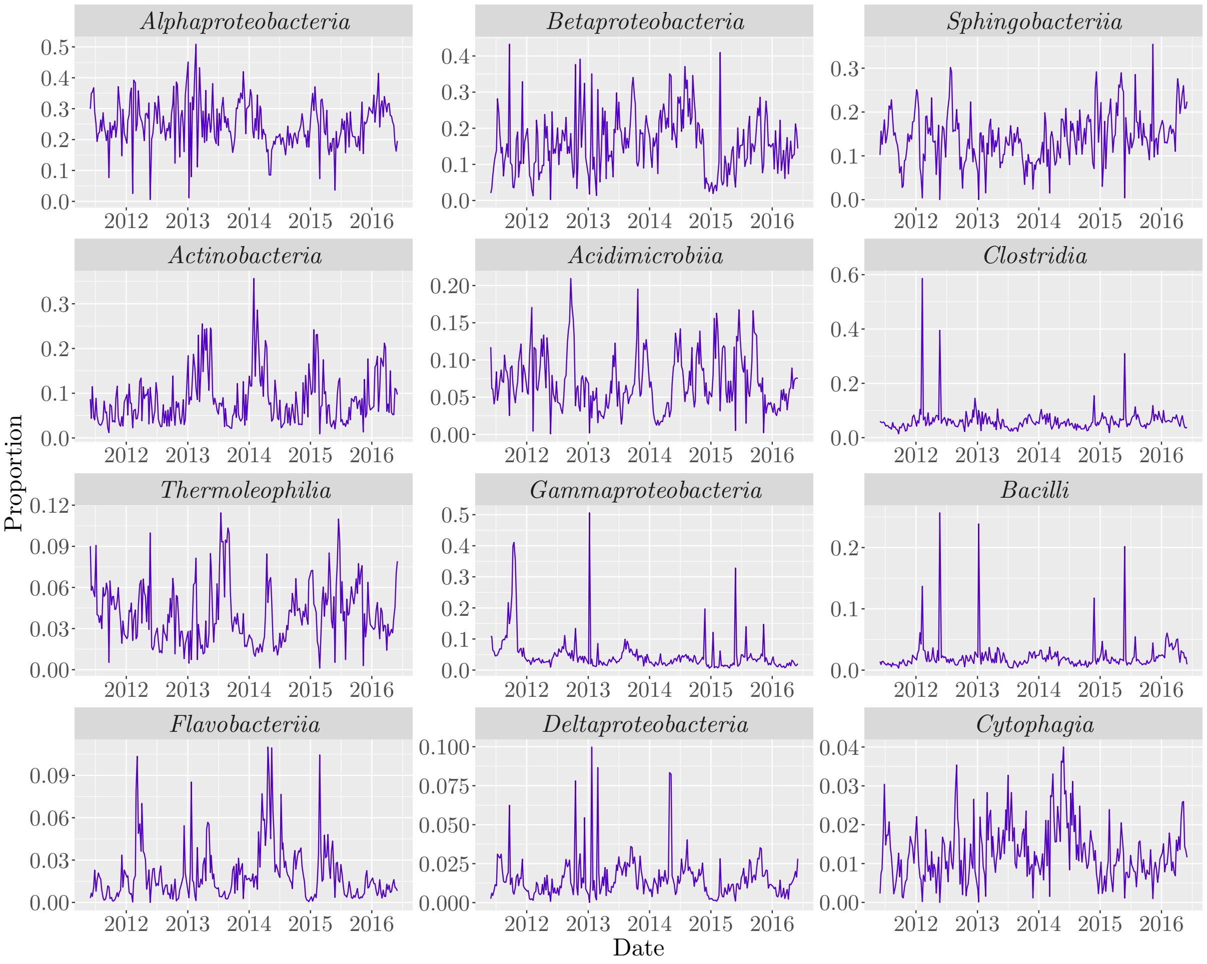


Figure 7: Time series plot for the top 12 classes based on median abundance.

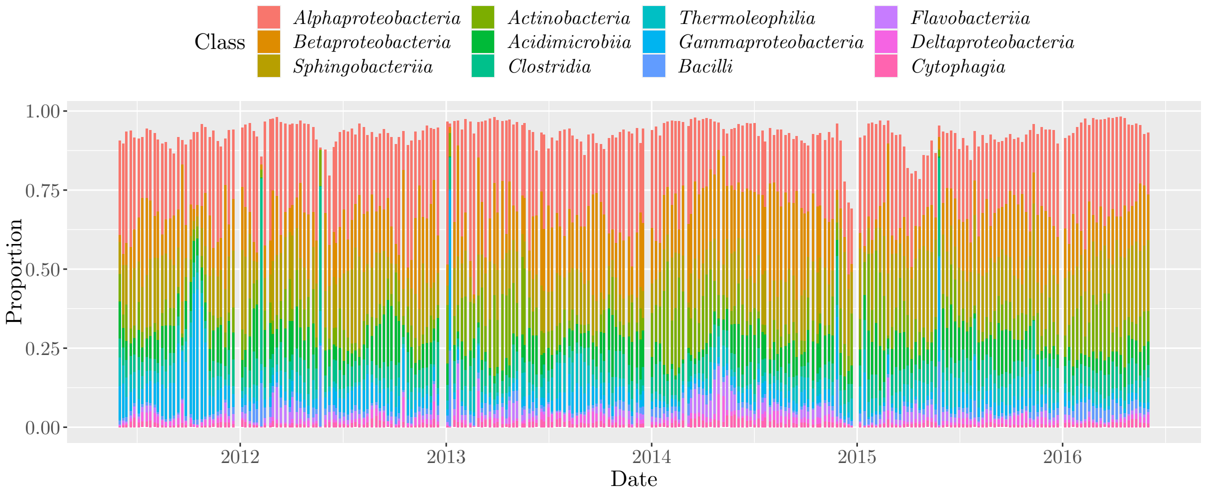


Figure 8: Stacked bar plot for the top 12 classes based on median abundance.

where $-\infty < \omega < \infty, \sigma_0^{-2} > 2\,|\omega|$, which is equivalent to $\varpi_0 > 0, \varpi_1 > 0$.

# 4 Simulation study

## 4.1 Description

Here we give the details of the simulation study designed to compare the performance of different shrinkage priors in a VAR(1) model. We compare the standard horseshoe, regularised horseshoe and the spike-and-slab. Additionally, we perform inference with an independent normal prior for each element of the autoregressive matrix, that is

$$a_{jk} \sim \mathrm{N}(c, d^2) \qquad j = 1, \dots, K, \ k = 1, \dots K,$$

to see the effect of choosing a prior that does not encourage shrinkage. The horseshoe prior is described in (10) of Section 5.1 of the main text and the regularised horseshoe prior is described in (18) of Section 5.3 of the main text. Here we briefly describe the spike-and-slab prior.

As mentioned in the preamble to Section 5 of the main text, the spike-and-slab prior is a zero-mean scale-mixture of normals with a discrete mixing distribution. A spike-and-slab prior for a VAR(1) model is given by

$$\begin{aligned} a_{jk}|\lambda_{jk}, d &\sim \lambda_{jk}\mathrm{N}(0, d^2) + (1 - \lambda_{jk})\delta_0, \\ \lambda_{jk} &\sim \mathrm{Bern}(\psi_{jk}), \qquad j = 1, \dots, K, \ k = 1, \dots, K, \end{aligned}$$

where the indicator variable $\lambda_{jk} \in \{0, 1\}$ denotes the presence ($\lambda_{jk} = 1$) or absence ($\lambda_{jk} = 0$) of autoregressive coefficient $a_{jk}$. In the simulation study, we fit the model with a spike-and-slab prior by introducing an auxiliary variable called the effect size $\tilde{a}_{jk}$ (see O'Hara and Sillanpää (2009)) and setting $a_{jk} = \tilde{a}_{jk}\lambda_{jk}$. We assume that the indicators and effects are independent *a priori*, which is the approach of Kuo and Mallick (1998), that is $\pi(\tilde{a}_{jk}, \lambda_{jk}) = \pi(\tilde{a}_{jk})\pi(\lambda_{jk})$.

We simulate three autoregressive coefficient matrices constrained to the stationary region, with $K = 12$ and varying degrees of sparsity, $\mathrm{A}_{80}$, $\mathrm{A}_{50}$ and $\mathrm{A}_{20}$, where the subscripts indicate the rough percentage of zero-coefficients in the matrix. Their corresponding heatmaps are shown in Figures 9 to 11. Our simulated data have 250 time points so that the dimensions roughly match the dimensions of our clustered WWTP data.

We assume a time invariant mean and adopt the simple diagonal error structure with common variance $\sigma^2 = 1$ for the simulation study. Hyperparameters for the priors on A are chosen so that the conditional expectations and variances are the same (or similar). All of our priors have a conditional expectation of zero. It can be shown that the conditional variance under the spike-and-slab prior is $\mathrm{Var}\left(a_{jk}|d, \psi_{jk}\right) = d^2\psi_{jk}$ and under both the standard horseshoe and regularised horseshoe prior is undefined. The variance under the normal prior is simply $d^2$. Therefore, we choose $\psi_{jk} = 0.5$ for all $j, k$ and $d^2 = 200$ in the spike-and-slab prior and $d^2 = 100$ in the normal prior, resulting in reasonably large (conditional) variances of 100.

`Stan` is used to fit the majority of models, with the exception of the spike-and-slab prior, as `Stan` is only suitable for fitting models with continuous valued parameters. Instead, a Gibbs sampler is written in `R` to fit the VAR(1) model with a spike-and-slab prior for A. The Gibbs sampler alternates between updating all of the effect sizes $\tilde{\boldsymbol{a}} = \mathrm{vec}(\tilde{A})$ together and updating all of the indicator variables one at a time in a random order from their full conditional distributions (FCDs).

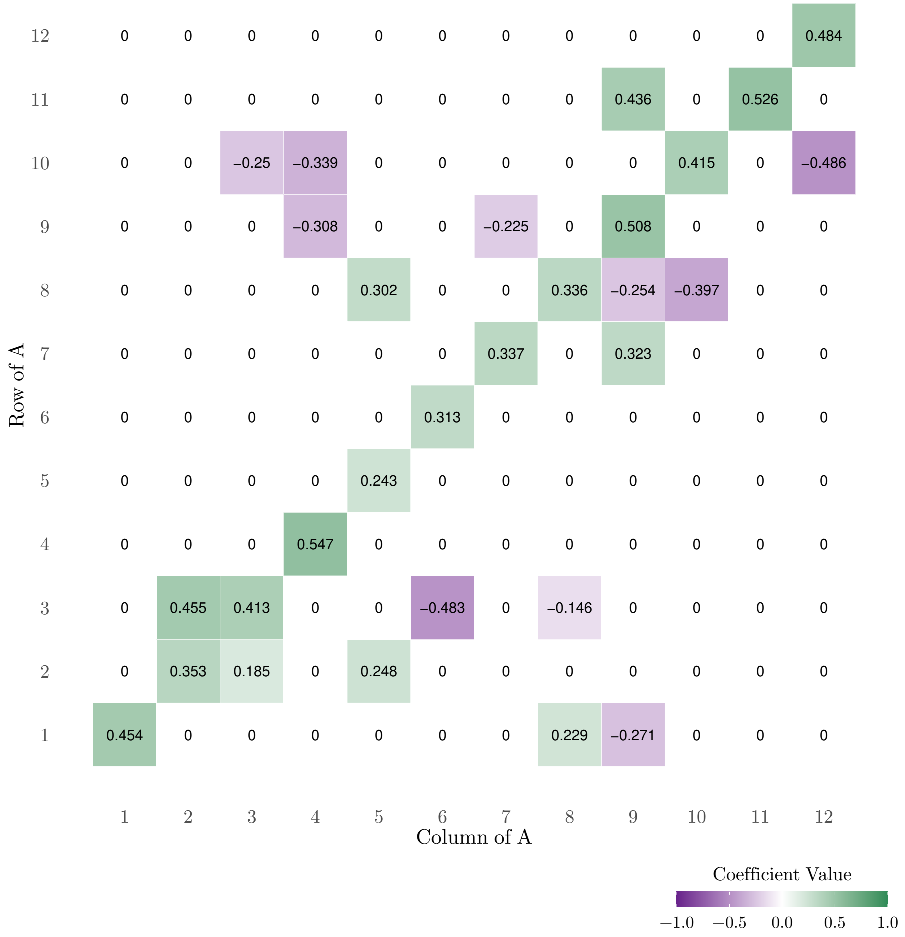


Figure 9: Heatmap of $A_{80}$.

Let $\boldsymbol{z}_t = \boldsymbol{y}_t - \boldsymbol{\mu}$ and $\mathrm{Z} = \begin{pmatrix} \boldsymbol{z}_1^T \\ \vdots \\ \boldsymbol{z}_N^T \end{pmatrix}$. Then the FCD for $\tilde{\boldsymbol{a}}$ when $\Sigma = \sigma^2 \mathrm{I}_K$ is given by

$$
\begin{aligned}
&\tilde{\boldsymbol{a}} | \mathrm{Z}, \Lambda, \Sigma \sim \mathrm{N}_{K^2}(\boldsymbol{M}_{\tilde{a}}, \mathrm{V}_{\tilde{a}}), \text{ where} \\
&\qquad \mathrm{V}_{\tilde{a}} = \operatorname{blockdiag}\left\{ \left( d^{-2}\mathrm{I}_K + \sigma^{-2} {\mathrm{Z}_{t-1}^{1*}}^T \mathrm{Z}_{t-1}^{1*} \right)^{-1}, \dots, \left( d^{-2}\mathrm{I}_K + \sigma^{-2} {\mathrm{Z}_{t-1}^{K*}}^T \mathrm{Z}_{t-1}^{K*} \right)^{-1} \right\}, \\
&\qquad \boldsymbol{M}_{\tilde{a}} = \begin{bmatrix} \left( d^{-2}\mathrm{I}_K + \sigma^{-2} {\mathrm{Z}_{t-1}^{1*}}^T \mathrm{Z}_{t-1}^{1*} \right)^{-1} \sigma^{-2} {\mathrm{Z}_{t-1}^{1*}}^T \boldsymbol{z}_{2:N,1} \\ \vdots \\ \left( d^{-2}\mathrm{I}_K + \sigma^{-2} {\mathrm{Z}_{t-1}^{K*}}^T \mathrm{Z}_{t-1}^{K*} \right)^{-1} \sigma^{-2} {\mathrm{Z}_{t-1}^{K*}}^T \boldsymbol{z}_{2:N,K} \end{bmatrix},
\end{aligned}
$$

with $\mathrm{Z}_{t-1}^{j*} = (\lambda_{j1}\mathrm{Z}_{1:N-1,1}, \dots, \lambda_{jK}\mathrm{Z}_{1:N-1,K})$, $\boldsymbol{z}_{2:N,k}$ is column $k$ of Z without its first row and $\mathrm{Z}_{1:N-1,k} = (z_{1k}, \dots, z_{N-1,K})^T$.

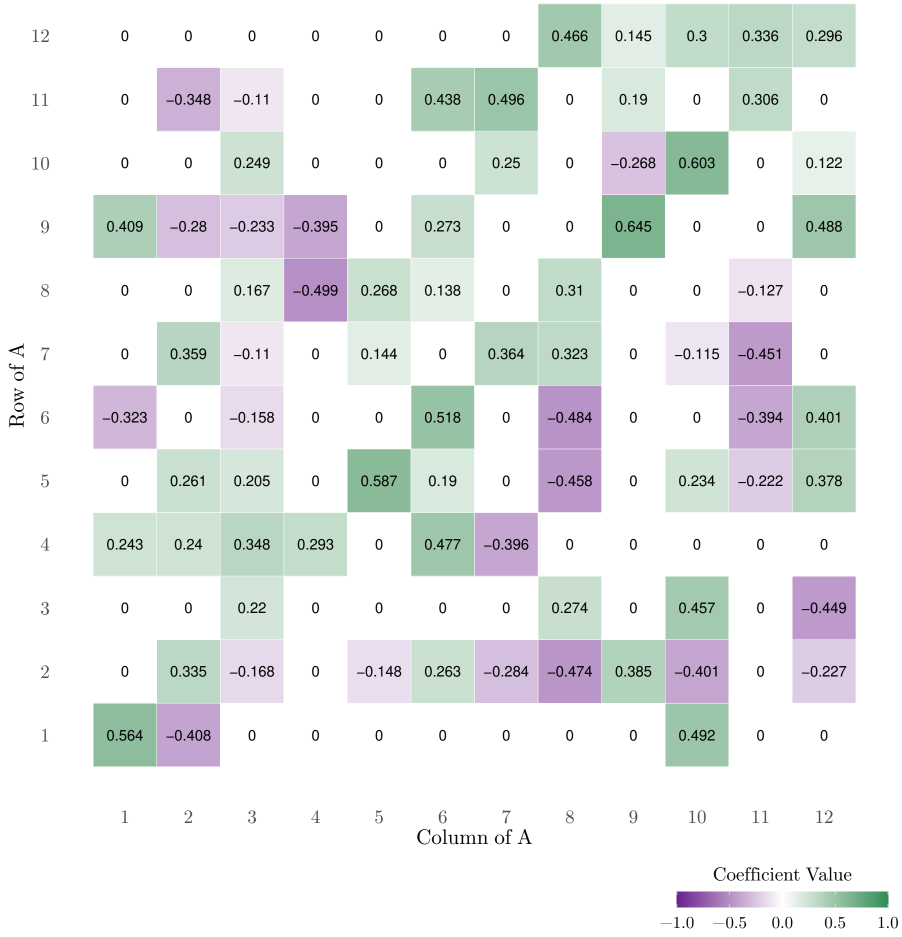


Figure 10: Heatmap of $A_{50}$.

Let $\mathrm{Z}_{t-1} = \begin{pmatrix} \boldsymbol{z}_1^T \\ \vdots \\ \boldsymbol{z}_{N-1}^T \end{pmatrix}$. Then the FCD for the $(j,k)$-th indicator parameter $\lambda_{jk}$ is given by

$$\begin{aligned} &\lambda_{jk}|\mathrm{Z} \sim \mathrm{Bern}(\tilde{p}_{jk}), \text{ with} \\ &\tilde{p}_{jk} = c_{jk} + (c_{jk} + d_{jk}), \text{ where} \\ &c_{jk} = p_{jk} \exp\left\{-\frac{1}{2\sigma^2}(\mathrm{Z}_{2:N,j} - \mathrm{Z}_{t-1}\boldsymbol{a}_j^*)^T(\mathrm{Z}_{2:N,j} - \mathrm{Z}_{t-1}\boldsymbol{a}_j^*)\right\} \text{ and} \\ &d_{jk} = (1-p_{jk}) \exp\left\{-\frac{1}{2\sigma^2}(\mathrm{Z}_{2:N,j} - \mathrm{Z}_{t-1}\boldsymbol{a}_j^{**})^T(\mathrm{Z}_{2:N,j} - \mathrm{Z}_{t-1}\boldsymbol{a}_j^{**})\right\}. \end{aligned}$$

Note that $\boldsymbol{a}_j^* = (a_{j1}, \ldots, a_{jK})^T$ and $\boldsymbol{a}_j^{**}$ is the same except its $k$-th component is replaced with 0.

The time invariant mean $\boldsymbol{\mu}$ and the precision of the errors $\tau$ are also updated by direct simulation from their FCDs. The results presented are based on 4000 near-uncorrelated samples from four chains (1000 per chain) initialised at different starting points.

## 4.2 Results

First we look at the results for the data simulated using the most sparse matrix $\mathrm{A}_{80}$. We make comparisons with plots of the posterior means and 95% credible intervals (CIs) for the elements

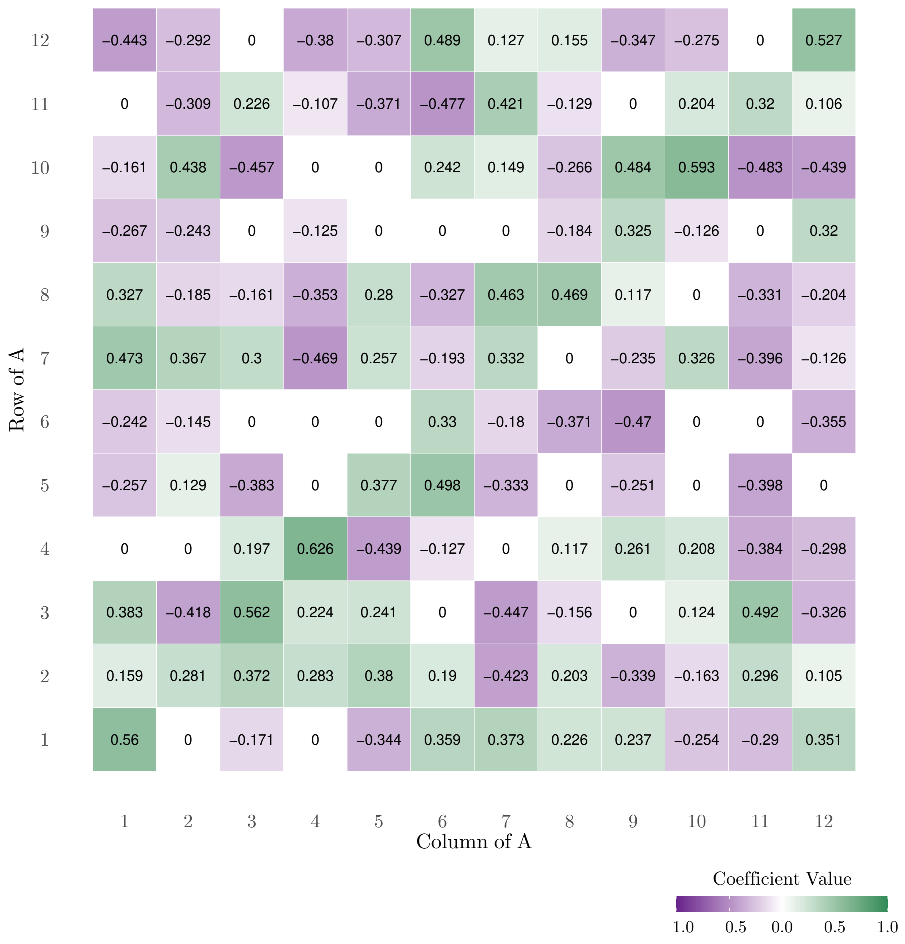


Figure 11: Heatmap of $A_{20}$.

of $A_{80}$, in the case of each prior. As a discriminator, we consider a non-zero coefficient incorrectly identified if its CI contains zero, likewise for a zero-coefficient if its CI does not contain zero. However, we emphasise that this does not necessarily mean that there is not support for a non-zero coefficient in the former case or a zero-coefficient in the latter case. With the normal prior, we can see in Figure 12 that most of the true values for the elements of $A_{80}$ are captured in the 95% CIs. However, for autoregressive coefficients $a_{8,12}$ and $a_{12,3}$, their true values of zero are not within the 95% CI. In addition to these, several other coefficients with true values of zero have CIs that only just include zero, for example, see $a_{10,7}$, $a_{11,10}$ and $a_{12,6}$. Given that there are a total of 144 parameters to infer, perhaps it is not surprising that the true values of some coefficients are not captured in the CIs.

Figure 13 shows the plot for the spike-and-slab prior for the 80% sparse matrix. Here most of the elements appear to be captured within their CIs, although $a_{2,5}$ does not have its true values contained within its CI. There is a suggestion of poor mixing in the non-zero elements, as $\lambda_{jk} = 1$ for 100% of the posterior samples. This is a suspiciously high percentage that may simply be the result of the sampler getting stuck at $\lambda_{jk} = 1$. The CIs are also extremely narrow for most of the zero elements. For the majority of these elements, $\lambda_{jk}$ is typically zero in $\sim 99\%$ of the posterior samples, which may also indicate poor mixing.

The results for the horseshoe prior are shown in Figure 14. All the true values for the autoregressive coefficients in $A_{80}$ have been captured in the CIs, except for one element, $a_{2,5}$, where the true value is just outside of the CI and zero is included. For many of the elements, the

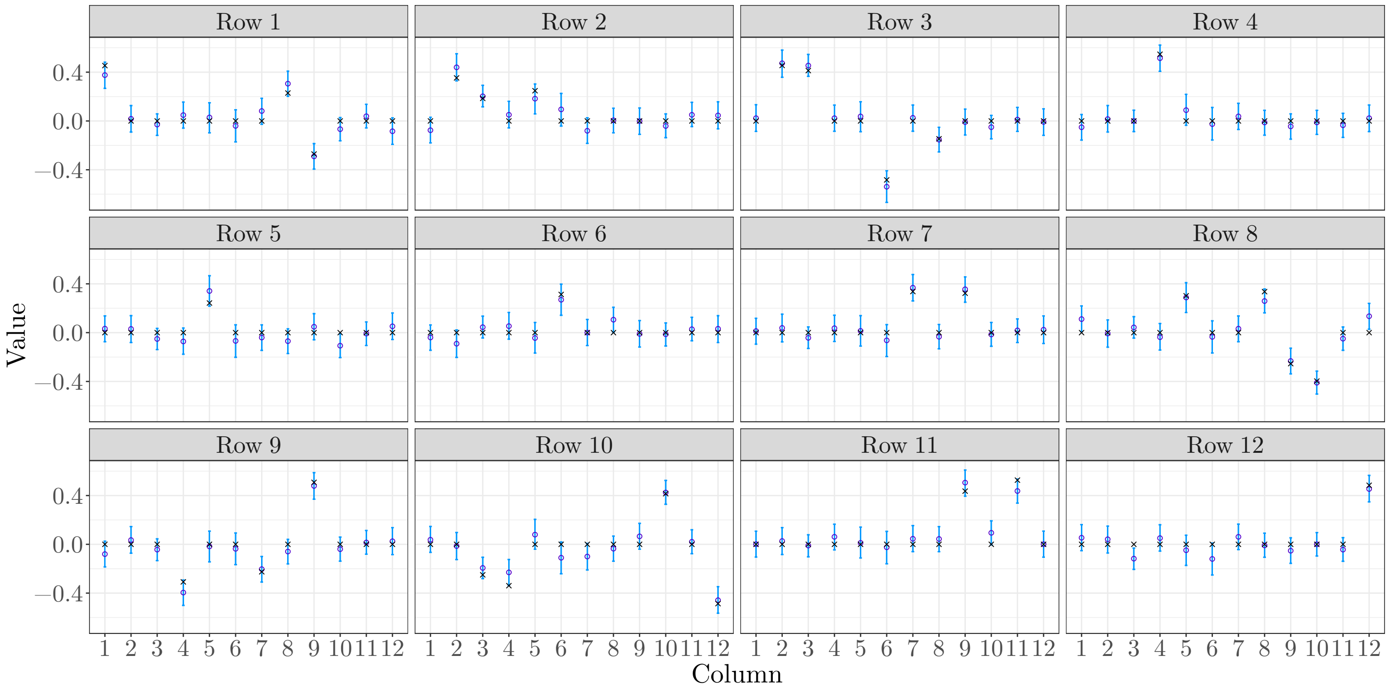


Figure 12: Posterior means (∘) and 95% credible intervals (—) for $A_{80}$, with the true values (×), under the multivariate normal prior.

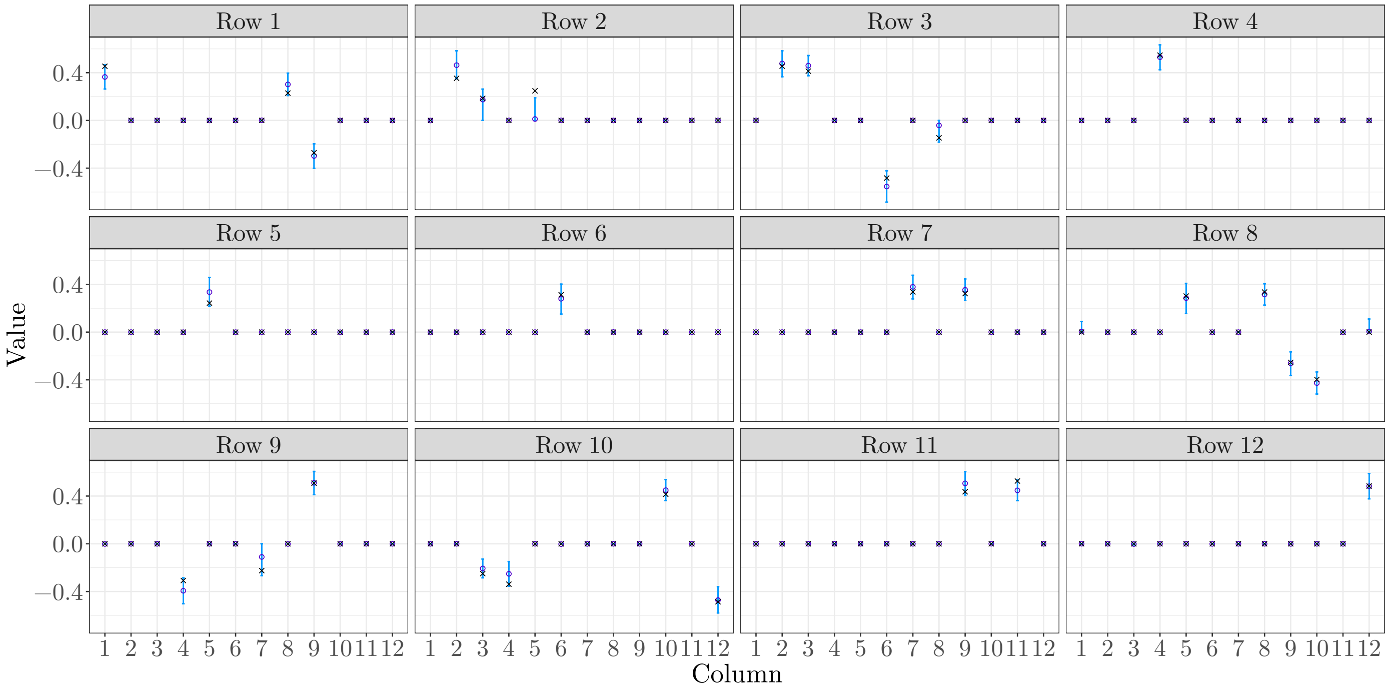


Figure 13: Posterior means (∘) and 95% credible intervals (—) for $A_{80}$, with the true values (×), under the spike-and-slab.

posterior means are very close to the true values, indicating a good performance by the horseshoe prior. However, even with the acceptance rate as 0.999 (which significantly reduces the step size used by the no-U-turn sampler (NUTS) in Stan), there were seven divergent transitions which is suggestive of a posterior whose curvature varies substantially across parameter space (see Hoffman and Gelman (2014); Stan Development Team (2020)). This indicates that some

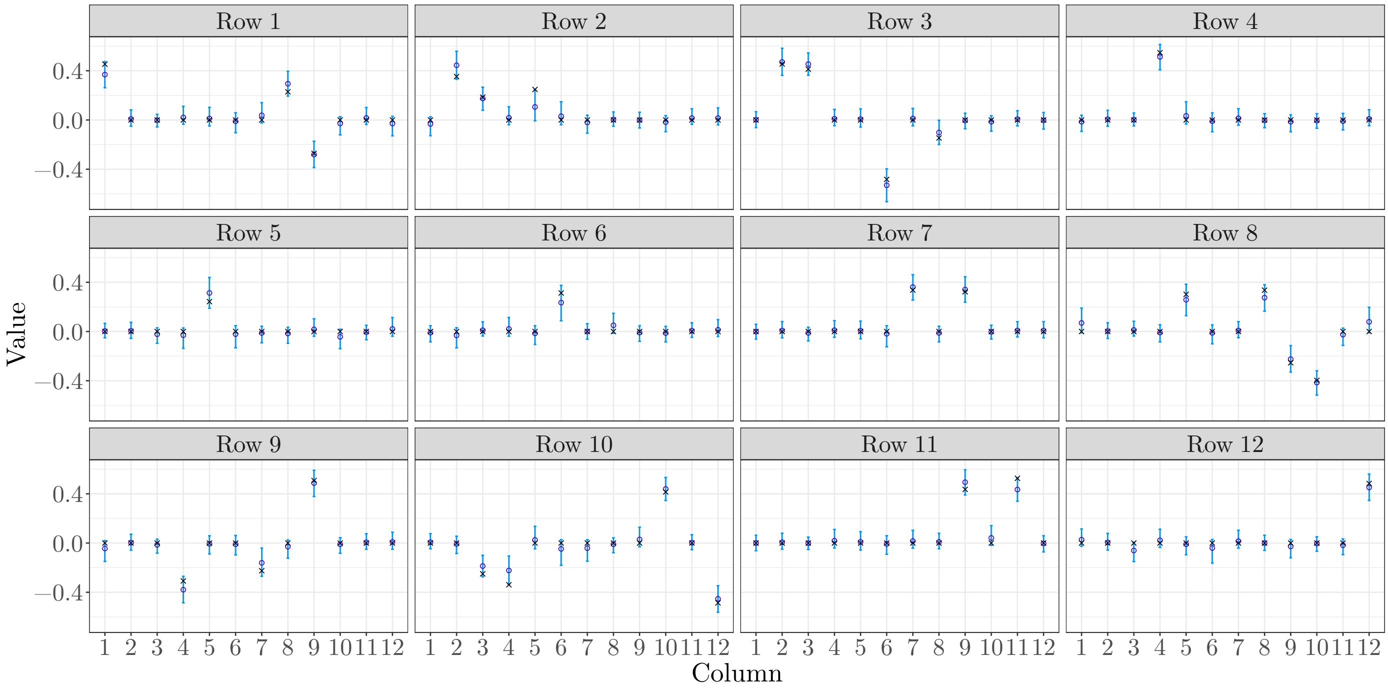


Figure 14: Posterior means (○) and 95% credible intervals (—) for $A_{80}$, with the true values (×), under the horseshoe prior.

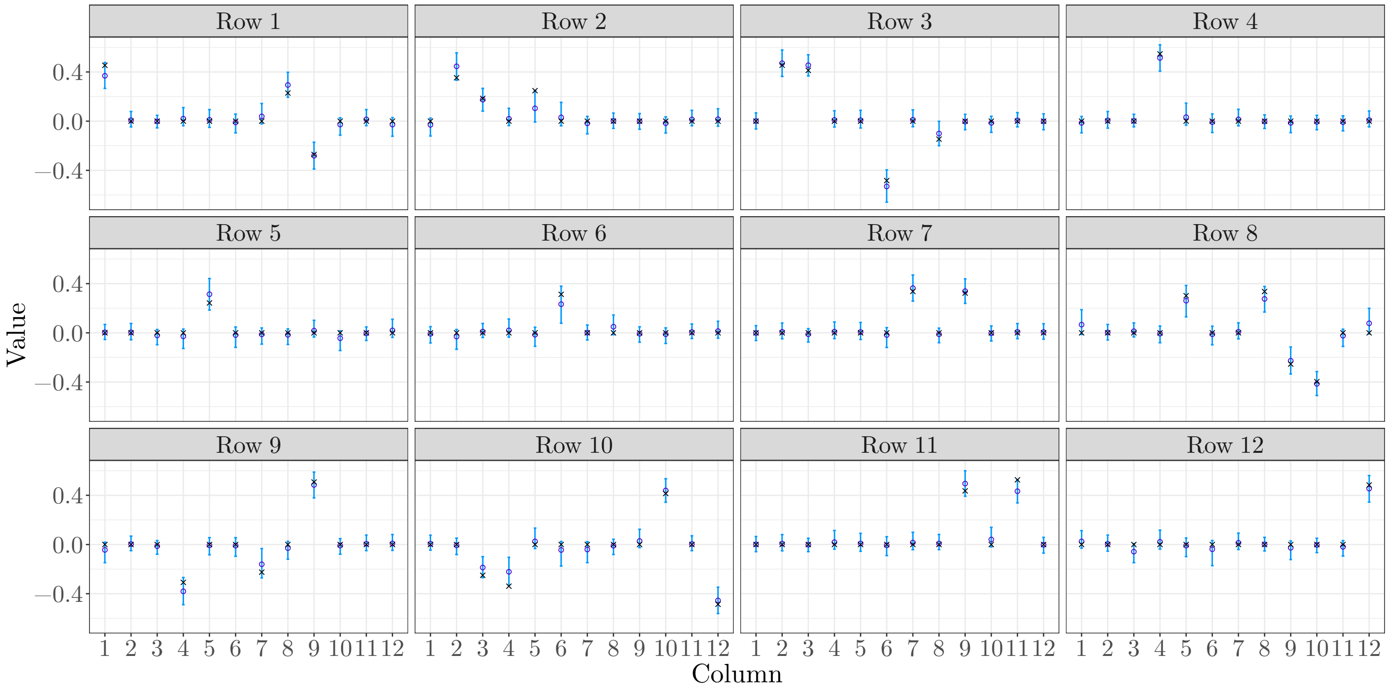


Figure 15: Posterior means (○) and 95% credible intervals (—) for $A_{80}$, with the true values (×), under the regularised horseshoe prior.

parts of posterior may be missed during sampling and the small step size causes an increase in computational time. This was not an issue for the regularised horseshoe prior, as larger step sizes could be used without yielding any divergent transitions. Figure 15 shows the results for the regularised horseshoe, which are very similar to the results obtained for the standard horseshoe prior. Although not obvious from the plot, the CI for $a_{2,5}$ contains the true value

of the element, but zero is included in the CI too. The obvious advantage here for using the regularised horseshoe instead of the standard horseshoe is computational speed. For example, running the model with the standard horseshoe with a smaller step size takes 26.5 minutes to perform 2000 iterations, whereas the regularised horseshoe with its larger step size (that results in zero divergent transitions) takes 10.5 minutes to perform the same number of iterations, which is more than twice as fast.

Next we compare the results of each prior for $A_{50}$ and begin again with the results of the multivariate normal prior, which are shown in Figure 16. Most elements have their true values captured in their posterior 95% CIs but we also note that $a_{1,12}, a_{2,11}$ and $a_{6,2}$ have their true values of zero outside of their CIs. This is most likely an effect of the prior not encouraging shrinkage. Although not obvious from the plot, the true value for $a_{9,2}$ also lies *just* outside of its CI.

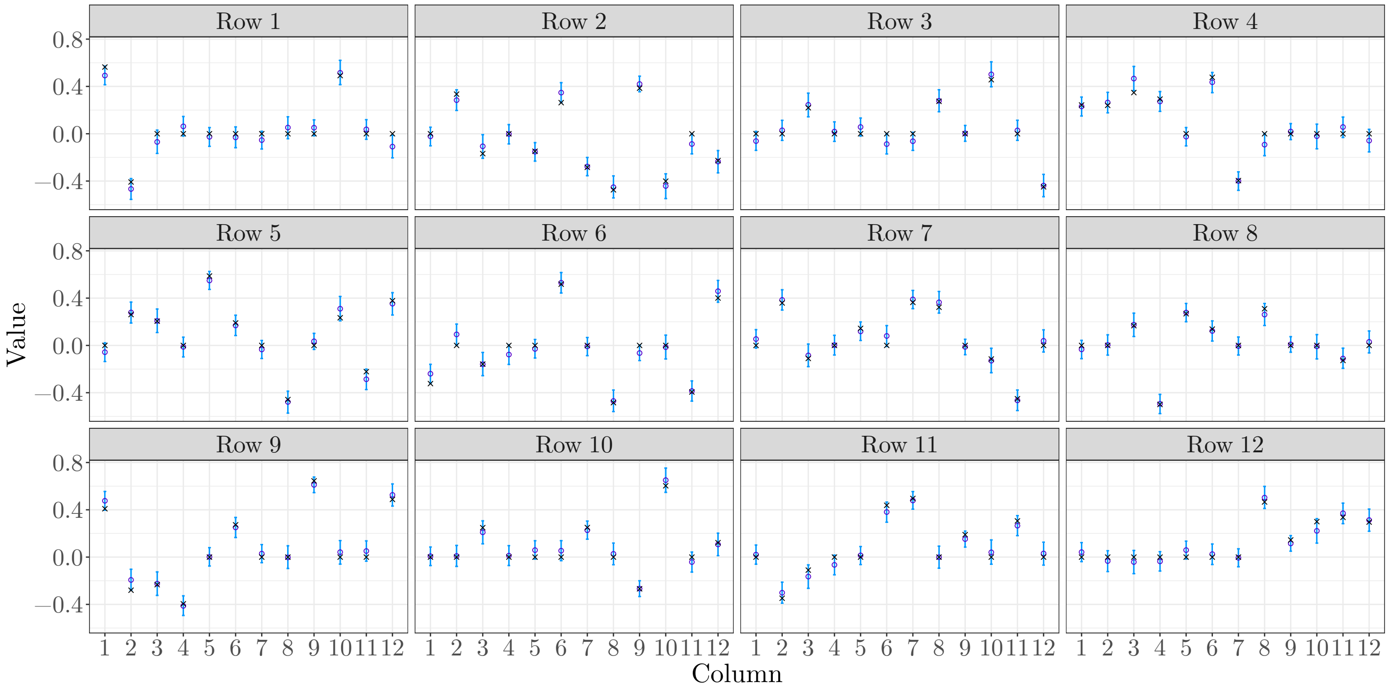


Figure 16: Posterior means (∘) and 95% credible intervals (—) for $A_{50}$, with the true values (×), under the multivariate normal prior.

The result for $A_{50}$ under the spike-and-slab prior are shown in Figure 17. The non-zero autoregressive coefficient $a_{11,3}$ contains zero in its CI. Additionally, the true values of $a_{2,3}$ (-0.168), $a_{8,11}$ (-0.127) and $a_{10,12}$ (0.122) are not captured in the posterior CIs, with their posterior means as zero. This could be due to their true values representing weak signals, which can be an issue when implementing models with spike-and-slab priors (for example, see the simulation study in Lei et al. (2011)). Almost 100% of the posterior samples for these elements are zero, for example, $\lambda_{10,12} = 0$ in $100\%, 100\%, 100\%$ and 98.8% of the posterior samples of each chain, respectively. Again, this may indicate "stickiness" of the sampler and hence poor mixing, as we saw with $A_{80}$. Furthermore, many of the other elements of $A_{50}$ suffer from this problem, for example, the majority of the remaining non-zero autoregressive coefficients have their corresponding $\lambda_{jk} = 1$ for 100% of their posterior samples.

Figure 18 shows the results for $A_{50}$ under the standard horseshoe prior. Again, the horseshoe seems to perform reasonably well and captures the true values of the autoregressive coefficients within the CIs, with the exception of $a_{9,2}$ and $a_{4,3}$. The true values of these elements lie just outside of the CIs. Comparing the results for $A_{50}$ under the regularised horseshoe (Figure 19) to the standard horseshoe, we can see that it performs similarly to the standard horseshoe.

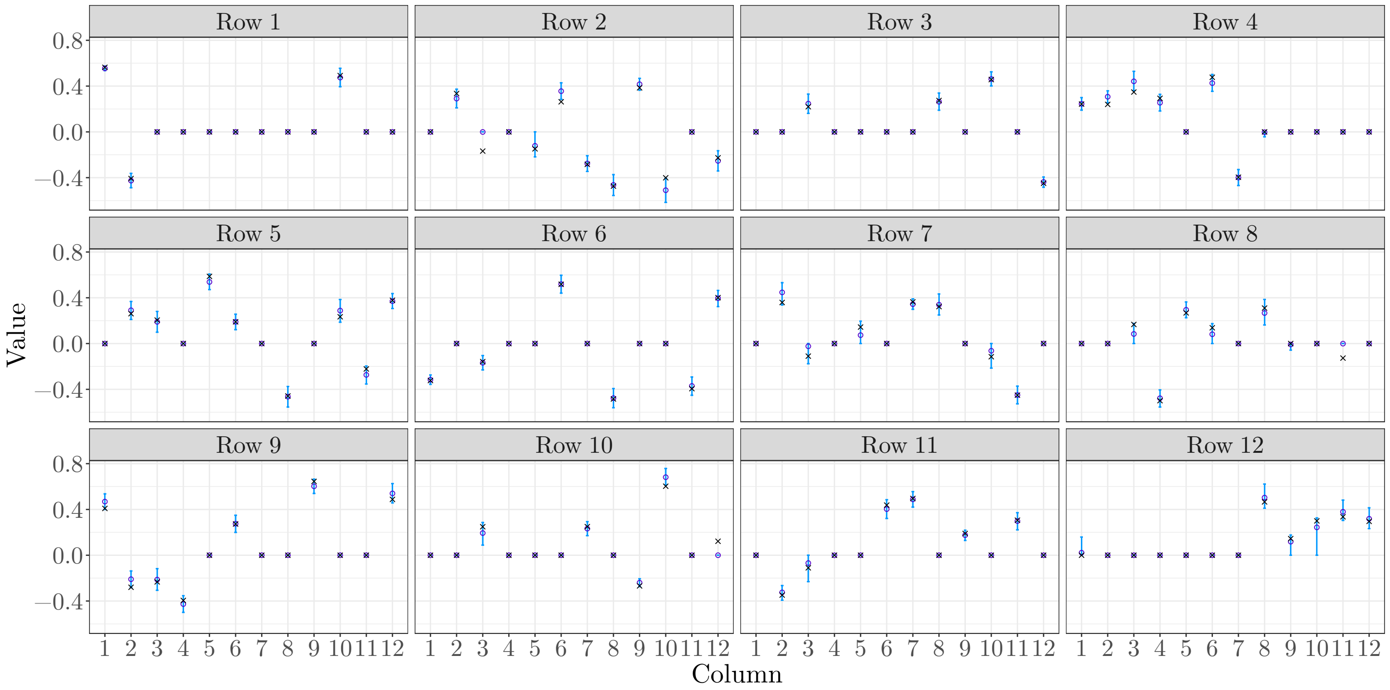


Figure 17: Posterior means (○) and 95% credible intervals (—) for $A_{50}$, with the true values (×), under the spike-and-slab.

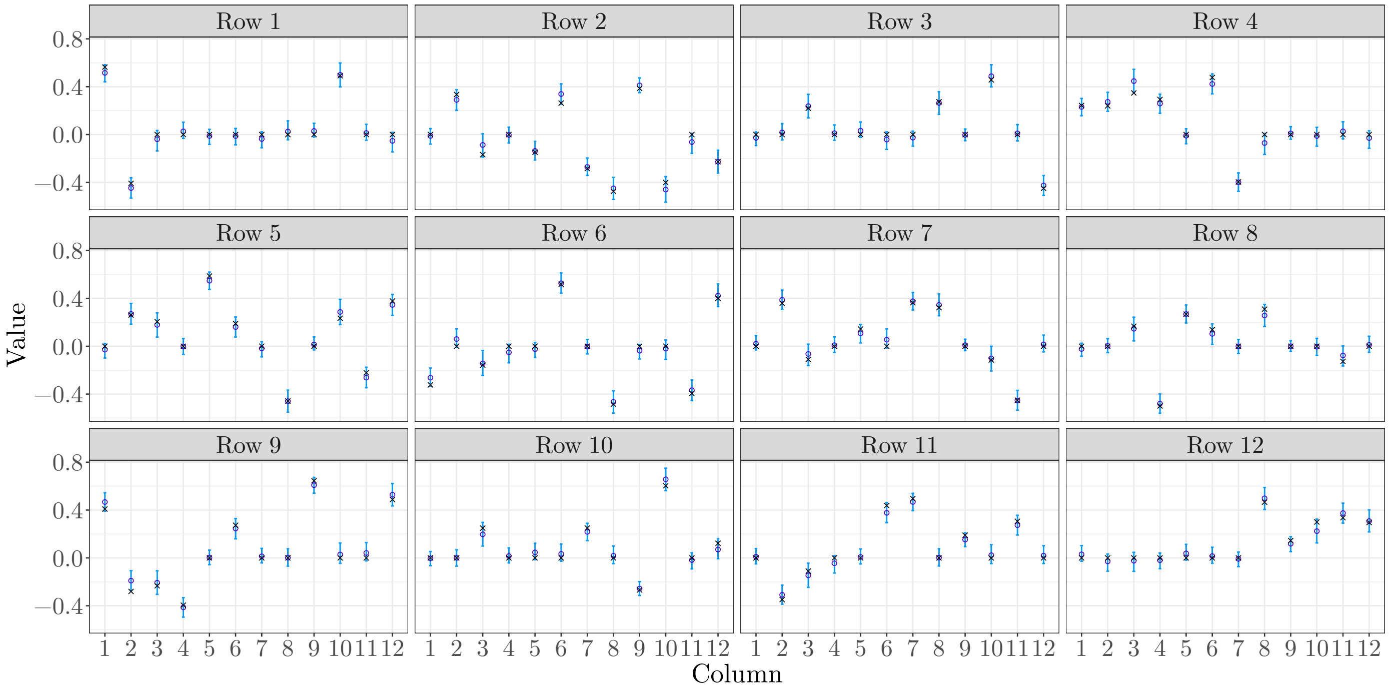


Figure 18: Posterior means (○) and 95% credible intervals (—) for $A_{50}$, with the true values (×), under the horseshoe prior.

However, the CI for $a_{9,2}$ does contain the true value. Additionally, we do not have any divergent transitions in our posterior samples when using the regularised horseshoe, whereas for the standard horseshoe, there were 41 divergent transitions.

Finally, we discuss the results for the simulation study with the least sparse matrix $A_{20}$. Figure 20 shows the results under the multivariate normal prior. Seven of the autoregressive

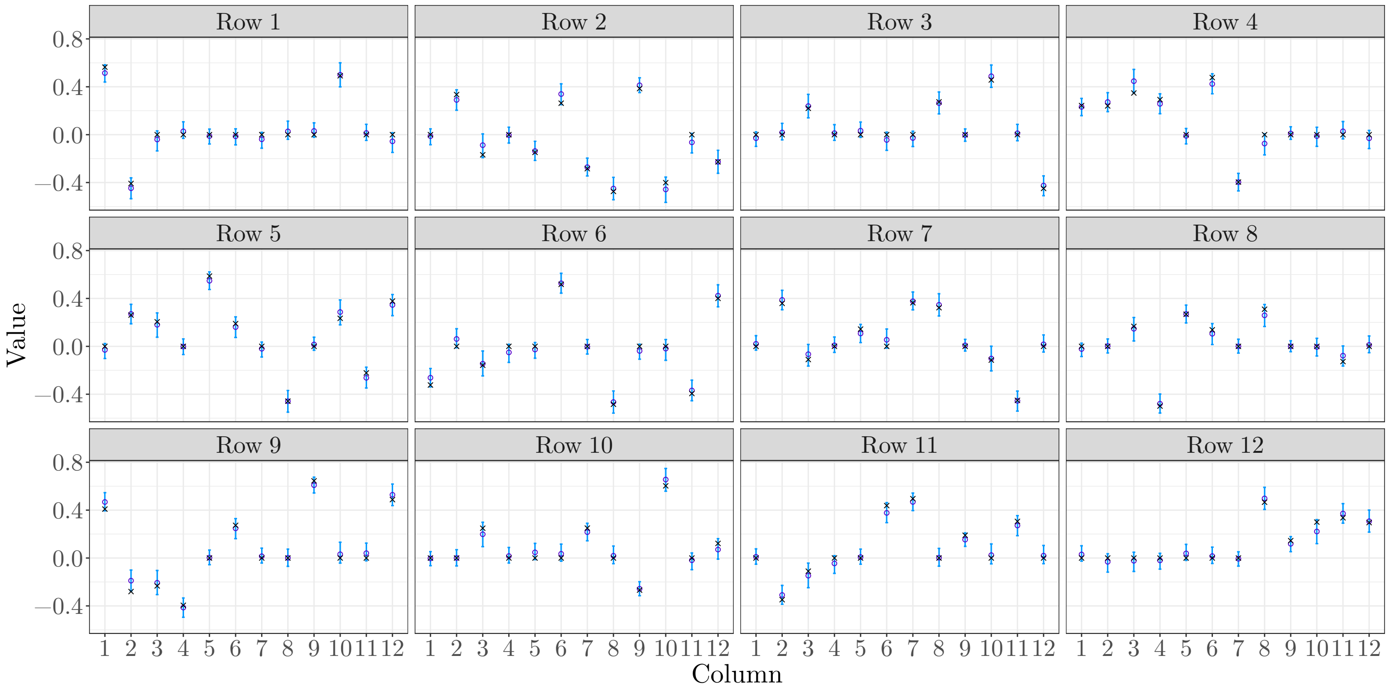


Figure 19: Posterior means (∘) and 95% credible intervals (—) for $A_{50}$, with the true values (×), under the regularised horseshoe prior.

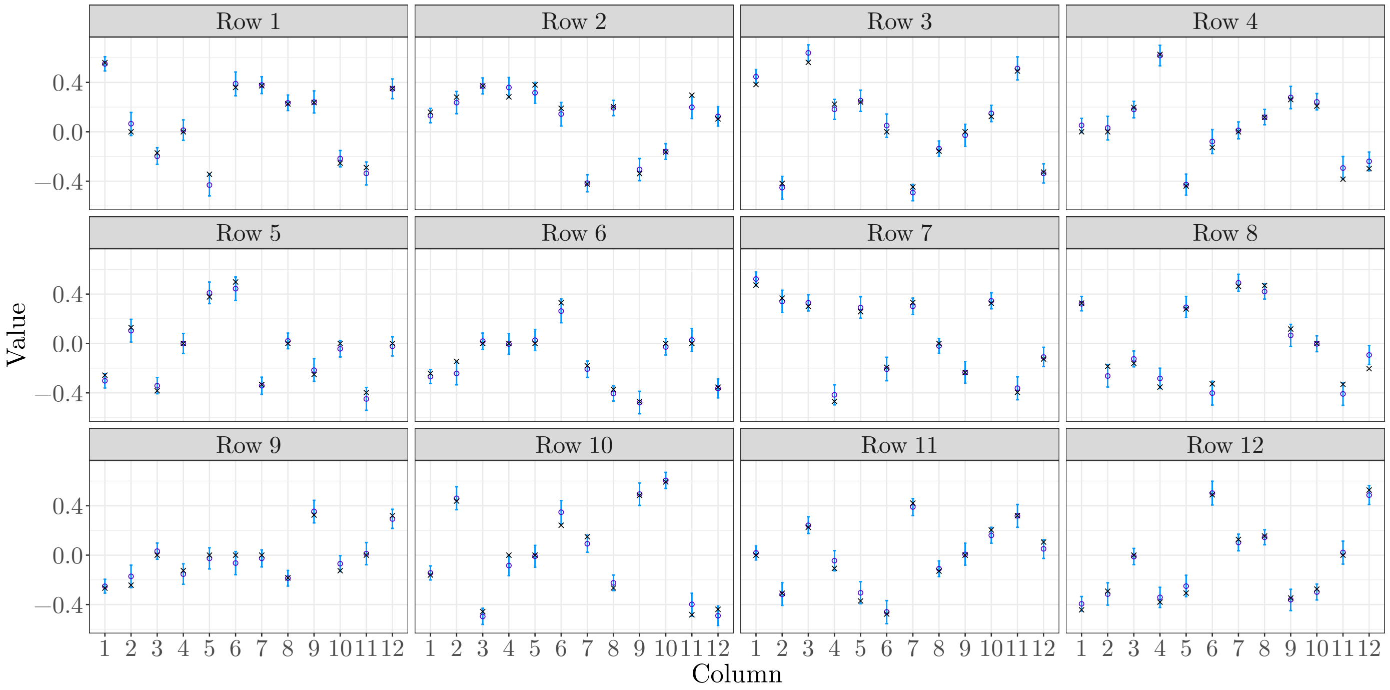


Figure 20: Posterior means (∘) and 95% credible intervals (—) for $A_{20}$, with the true values (×), under the multivariate normal prior.

coefficients ($a_{2,11}, a_{3,1}, a_{3,3}, a_{6,2}, a_{8,12}, a_{10,4}$ and $a_{10,6}$) do not have their true values in their CIs, although the true values lie just outside of the intervals. The multivariate normal prior only fails to "find" one of the zero-coefficients ($a_{10,4}$) but overall performs fairly well, as we might expect for this particular matrix.

Figure 21 shows the results for $A_{20}$ under the spike-and-slab prior. Clearly from the plots, the

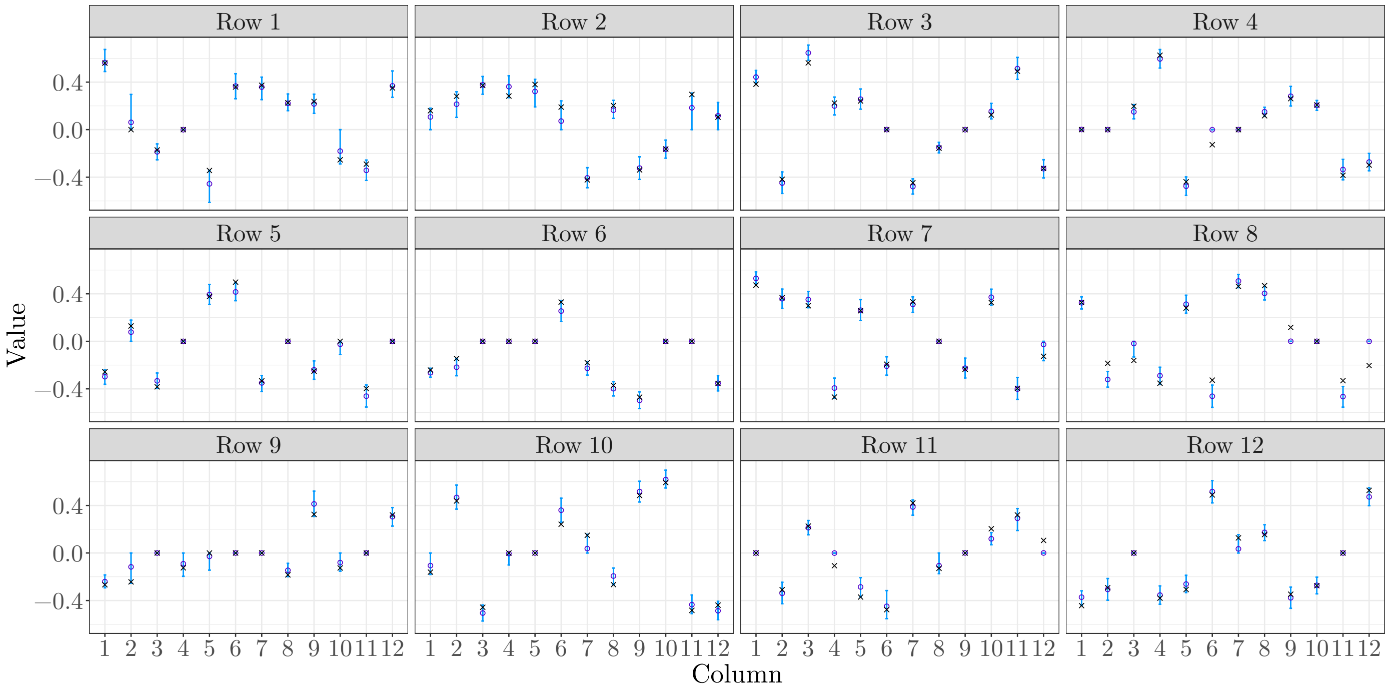


Figure 21: Posterior means (∘) and 95% credible intervals (—) for $A_{20}$, with the true values (×), under the spike-and-slab.

true values of many autoregressive coefficients have not been found, for example, $a_{4,6}$, $a_{8,9}$, $a_{8,12}$, $a_{11,4}$ and $a_{11,12}$ are all non-zero coefficients but zero is included in their CIs, meanwhile their true values are not included. Closer inspection reveals that 16 different autoregressive coefficients do not contain their true values in their CIs and 11 non-zero autoregressive coefficients include zero in their CIs. This is evidence to suggest that this prior is not well suited to data that break the assumption of sparsity. Furthermore, mixing issues are also likely to be a problem here, with many of the $\lambda_{jk}$ taking the same value for 100% of posterior samples in all four chains.

The standard horseshoe seems to perform better than the spike-and-slab prior when the data are simulated using $A_{20}$. However, inspecting the posterior means and CIs in Figure 22 clearly shows that $a_{8,12}$'s true value of $-0.204$ is not within the 95% CI. Further investigation reveals that seven other autoregressive coefficients do not have their true values contained in their corresponding CIs and $a_{11,12}$'s CI contains both the true value (0.106) and zero. As we found with the more sparse matrices, there were some divergent transitions (seven) present when using the standard horseshoe prior for $A_{20}$.

Finally, we discuss the results for $A_{20}$ under the regularised horseshoe prior. As we found with the more sparse autoregressive matrices, performance was similar to the standard horseshoe, although only six autoregressive coefficients did not have the correct value contained in their CIs. An almost identical result was also found for $a_{11,12}$ as the result found under the standard horseshoe, both the true non-zero value and zero were in the CI. For both this prior and the standard horseshoe, where there was evidence to suggest that the true values had not been identified by the model, most true values were very close to the edges of their CIs, which can be seen in Figure 23.

### 4.3 Summary

Table 4 shows the number of incorrectly identified autoregressive coefficients for each matrix and prior in the simulation study. Solely based on these results, if we have a matrix of autoregressive coefficients A in a VAR(1) model, where the level of sparsity is unknown (as we have with our

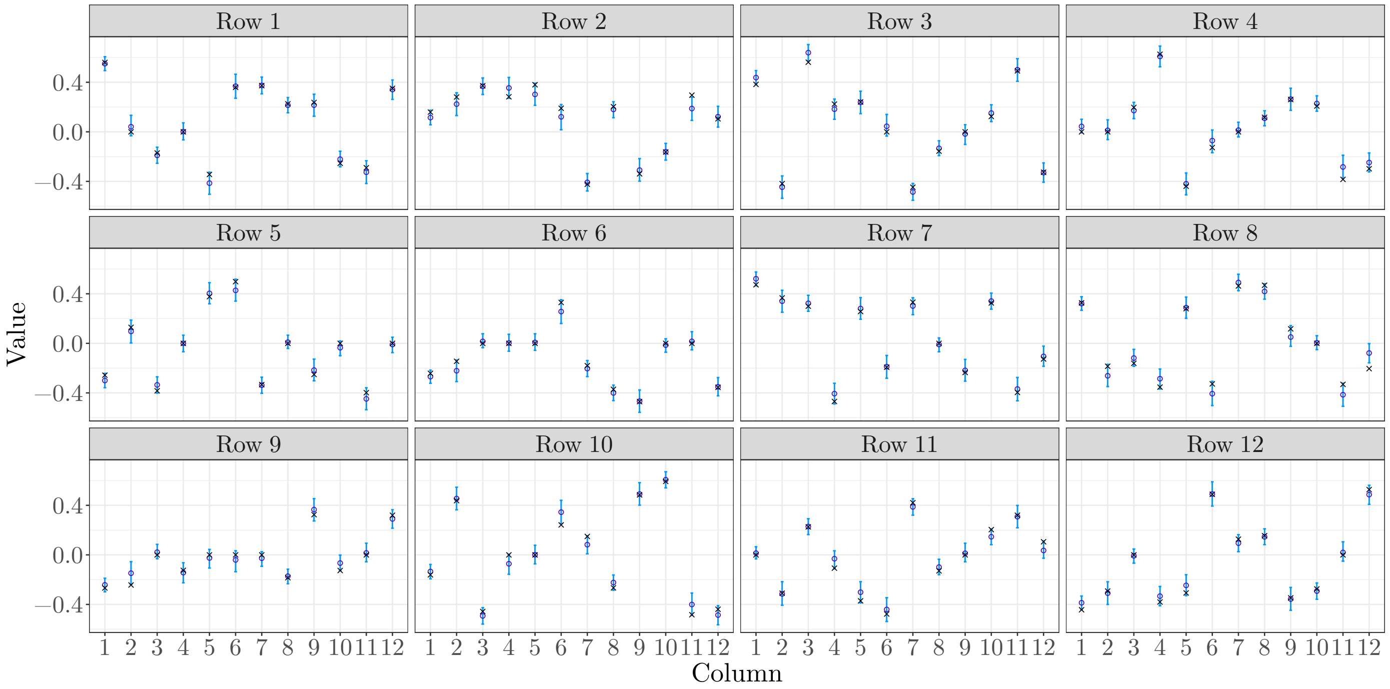


Figure 22: Posterior means (∘) and 95% credible intervals (—) for $A_{20}$, with the true values (×), under the horseshoe prior.

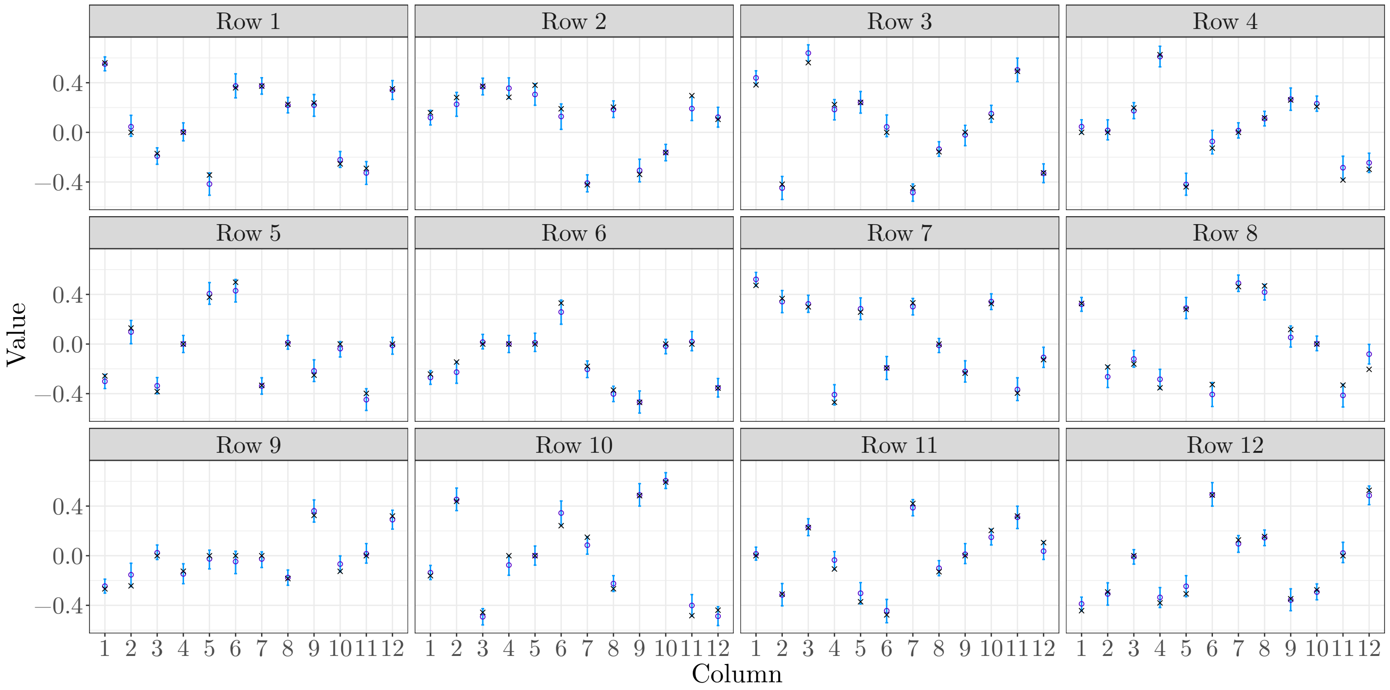


Figure 23: Posterior means (∘) and 95% credible intervals (—) for $A_{20}$, with the true values (×), under the regularised horseshoe prior.

WWTP data) then it would seem sensible to choose a regularised horseshoe prior for A. In the case where the data are simulated using $A_{50}$, the regularised horseshoe outperforms the other priors. For the data simulated with the least sparse matrix $A_{20}$, the regularised horseshoe performs as well as the multivariate normal. For the most sparse matrix, the spike-and-slab, standard horseshoe and regularised horseshoe only fail to correctly identify one coefficient $a_{2,5}$.

However, the regularised horseshoe does not have the sampling issues that the spike-and-slab prior has, nor does it suffer from the problem of divergent transitions that the standard horseshoe has. Furthermore, the regularised horseshoe performs computationally faster than the standard horseshoe, because the step size in the NUTS algorithm can be larger. The obvious choice for the prior for A in our model is the regularised horseshoe because of these benefits and also due to its flexibility with regards to varying degrees of sparseness in the autoregressive matrix.

| | **Prior** | | | |
|---|---|---|---|---|
| | Normal | Spike & Slab | Horseshoe | Regularised Horseshoe |
| $A_{80}$ | 2 | 1 | 1 | 1 |
| $A_{50}$ | 4 | 4 | 2 | 1 |
| $A_{20}$ | 7 | 27 | 8 | 7 |

Table 4: Number of autoregressive coefficients not correctly identified in the simulation study for each matrix and prior.

# 5 Prior for global shrinkage parameter

## 5.1 Derivation of conditional posterior for $\boldsymbol{a}^*$

The likelihood for Y in (9) in Section 5.1 in the main text is given by

$$\begin{aligned}\pi\left(\mathrm{Y}|\mathrm{A},\Sigma\right) &= \pi(\mathrm{E}|\Sigma)\\ &= (2\pi)^{-PQ/2}|\Sigma|^{-N/2}\exp\left\{-\frac{1}{2}\mathrm{tr}\left[\Sigma^{-1}(\mathrm{Y}-\mathrm{XA})^T(\mathrm{Y}-\mathrm{XA})\right]\right\}\\ &= (2\pi)^{-PQ/2}|\Sigma|^{-N/2}\\ &\quad\times\exp\left\{-\frac{1}{2}\mathrm{tr}\left[\Sigma^{-1}\left(\mathrm{Y}-\mathrm{X}\hat{\mathrm{A}}\right)^T\left(\mathrm{Y}-\mathrm{X}\hat{\mathrm{A}}\right)+\Sigma^{-1}\left(\mathrm{A}-\hat{\mathrm{A}}\right)^T\mathrm{X}^T\mathrm{X}\left(\mathrm{A}-\hat{\mathrm{A}}\right)\right]\right\},\end{aligned}$$

using the fact that $\hat{\mathrm{A}} = (\mathrm{X}^T\mathrm{X})^{-1}\mathrm{X}^T\mathrm{Y}$. The prior density for A is

$$\begin{aligned}\pi\left(\mathrm{A}\right) &= \pi\left(\boldsymbol{a}^*\right)\\ &= (2\pi)^{-PQ/2}|\tau^2\Lambda^*|^{-\frac{1}{2}}\exp\left\{-\frac{1}{2}\boldsymbol{a}^{*T}(\tau^2\Lambda^*)^{-1}\boldsymbol{a}^*\right\}.\end{aligned}$$

The posterior density for A is proportional to $\pi(\mathrm{A})\pi(\mathrm{Y}|\mathrm{A},\Sigma)$. Note that

$$\pi(\mathrm{Y}|\mathrm{A},\Sigma) \propto (2\pi)^{-PQ/2}|\Sigma|^{-N/2}\times\exp\left\{-\frac{1}{2}\mathrm{tr}\left[\Sigma^{-1}\left(\mathrm{A}-\hat{\mathrm{A}}\right)^T\mathrm{X}^T\mathrm{X}\left(\mathrm{A}-\hat{\mathrm{A}}\right)\right]\right\}.$$

We wish to find $\pi(\boldsymbol{a}^*|\mathrm{Y},\Sigma,\Lambda^*,\tau) \propto \pi(\boldsymbol{a}^*)\pi(\mathrm{Y}|\boldsymbol{a}^*,\Sigma,\Lambda^*,\tau)$. Up to a constant of proportionality the likelihood $\pi(\mathrm{Y}|\boldsymbol{a}^*,\Sigma,\Lambda^*,\tau)$ can be written as

$$\exp\left\{-\frac{1}{2}\left(\boldsymbol{a}^*-\hat{\boldsymbol{a}}^*\right)^T\left(\left(\mathrm{X}^T\mathrm{X}\right)^{-1}\otimes\Sigma\right)^{-1}\left(\boldsymbol{a}^*-\hat{\boldsymbol{a}}^*\right)\right\}.$$

Thus we have

$$\begin{aligned}&\pi(\mathrm{Y}|\boldsymbol{a}^*,\Sigma,\Lambda^*,\tau)\\ &\qquad\propto\exp\left\{-\frac{1}{2}\left(\boldsymbol{a}^{*T}\left(\left(\mathrm{X}^T\mathrm{X}\right)^{-1}\otimes\Sigma\right)^{-1}\boldsymbol{a}^*\right)-2\boldsymbol{a}^{*T}\left(\left(\mathrm{X}^T\mathrm{X}\right)^{-1}\otimes\Sigma\right)^{-1}\hat{\boldsymbol{a}}^*\right\}.\end{aligned}$$

The posterior density for $\boldsymbol{a}^*$ is given by

$$\begin{aligned}
&\pi(\boldsymbol{a}^*|\mathrm{Y}, \Sigma, \Lambda^*, \tau) \\
&\quad \propto \exp\left\{-\frac{1}{2}\boldsymbol{a}^{*T}(\tau^2\Lambda^*)^{-1}\boldsymbol{a}^*\right\} \\
&\qquad \times \exp\left\{-\frac{1}{2}\left(\boldsymbol{a}^{*T}\left(\left(\mathrm{X}^T\mathrm{X}\right)^{-1}\otimes\Sigma\right)^{-1}\boldsymbol{a}^*\right) - 2\boldsymbol{a}^{*T}\left(\left(\mathrm{X}^T\mathrm{X}\right)^{-1}\otimes\Sigma\right)^{-1}\hat{\boldsymbol{a}}^*\right\}. \\
&\quad = \exp\left\{-\frac{1}{2}\left[\boldsymbol{a}^{*T}\left((\tau^2\Lambda^*)^{-1} + \left(\left(\mathrm{X}^T\mathrm{X}\right)^{-1}\otimes\Sigma\right)^{-1}\right)\boldsymbol{a}^*\right.\right. \\
&\qquad \left.\left. - 2\boldsymbol{a}^{*T}\left(\left(\mathrm{X}^T\mathrm{X}\right)^{-1}\otimes\Sigma\right)^{-1}\hat{\boldsymbol{a}}^*\right]\right\}.
\end{aligned}$$

This is the density corresponding to the posterior distribution given in (11) in Section 5.1 of the main text.

## 5.2 Derivation of $\mathcal{K}_j$ for other parametric forms of $\Sigma$

### 5.2.1 Compound symmetric $\Sigma$

The compound symmetric variance matrix can be written as $\Sigma = \rho\sigma^2(\mathbf{1}_Q\mathbf{1}_Q^T + (1-\rho)/\rho\mathrm{I}_Q)$, where $\sigma^2 > 0$ and $\mathbf{1}_Q$ is a $Q$-vector of 1s. The eigenvalues of $\mathbf{1}_Q\mathbf{1}_Q^T$ are $Q$ and 0 and so the eigenvalues of $\Sigma$ are $\rho\sigma^2\left(Q + (1-\rho)/\rho\right)$ and $\sigma^2(1-\rho)$. Therefore, $\Sigma$ is positive definite if and only if

$$\rho\left(Q + \frac{1-\rho}{\rho}\right) > 0 \iff \rho > -\frac{1}{Q-1}$$

and

$$1-\rho > 0 \iff \rho < 1,$$

i.e. $-1/\left(Q-1\right) < \rho < 1$.

To derive the shrinkage factor matrix in the case of a compound symmetric variance matrix, we need to first calculate the precision matrix $\Sigma^{-1}$. This is found by application of the Sherman-Morrison formula, that is

$$(\mathrm{A} + \boldsymbol{u}\boldsymbol{v}^T)^{-1} = \mathrm{A}^{-1} - \frac{\mathrm{A}^{-1}\boldsymbol{u}\boldsymbol{v}^T\mathrm{A}^{-1}}{1 + \boldsymbol{v}^T\mathrm{A}^{-1}\boldsymbol{u}}, \tag{4}$$

where $\mathrm{A} \in \mathbb{R}^{Q\times Q}$ is an invertible square matrix and $\boldsymbol{u}, \boldsymbol{v} \in \mathbb{R}^Q$ are vectors. Here $\boldsymbol{u}\boldsymbol{v}^T$ is the outer product of $\boldsymbol{u}$ and $\boldsymbol{v}$ and $(1 + \boldsymbol{v}^T\mathrm{A}^{-1}\boldsymbol{u}) \neq 0$. We note that the variance matrix can be written as $\Sigma = \rho\sigma^2\mathbf{1}_Q\mathbf{1}_Q^T + \sigma^2(1-\rho)\mathrm{I}_Q$. Substituting $\boldsymbol{u} = \rho\sigma^2\mathbf{1}_Q$, $\boldsymbol{v} = \mathbf{1}_Q$ and $\mathrm{A} = \sigma^2(1-\rho)\mathrm{I}_Q$ into equation (4) above, we can show that the precision matrix is

$$\begin{aligned}
\Sigma^{-1} &= \frac{1}{\sigma^2(1-\rho)}\mathrm{I}_Q - \frac{\left(\frac{1}{\sigma^2(1-\rho)}\right)\left(\frac{\rho\sigma^2}{\sigma^2(1-\rho)}\right)\mathbf{1}_Q\mathbf{1}_Q^T}{1 + \mathbf{1}_Q^T\frac{1}{\sigma^2(1-\rho)}\mathrm{I}_Q\rho\sigma^2\mathbf{1}_Q} \\
&= \frac{1}{\sigma^2(1-\rho)}\mathrm{I}_Q - \frac{\frac{\rho}{\sigma^2(1-\rho)^2}\mathbf{1}_Q\mathbf{1}_Q^T}{1 + \frac{Q\rho}{1-\rho}} \\
&= \frac{1}{\sigma^2(1-\rho)}\mathrm{I}_Q - \left(\frac{\rho}{\sigma^2(1-\rho)^2}\right)\left(\frac{1-\rho}{1-\rho+Q\rho}\right)\mathbf{1}_Q\mathbf{1}_Q^T \\
&= \frac{1}{\sigma^2(1-\rho)}\left\{\mathrm{I}_Q - \frac{\rho}{1+\rho(Q-1)}\mathbf{1}_Q\mathbf{1}_Q^T\right\}.
\end{aligned}$$

Now we can write the shrinkage factor matrix as

$$\begin{aligned}
\mathcal{K}_j &= \left(\mathrm{I}_Q + Ns_j^2\tau^2\Lambda_j\Sigma^{-1}\right)^{-1} \\
&= \left[\mathrm{I}_Q + \frac{Ns_j^2\tau^2}{\sigma^2(1-\rho)}\Lambda_j\left(\mathrm{I}_Q - \frac{\rho}{1+\rho(Q-1)}\mathbf{1}_Q\mathbf{1}_Q^T\right)\right]^{-1} \\
&= \left[\mathrm{I}_Q + \frac{Ns_j^2\tau^2}{\sigma^2(1-\rho)}\Lambda_j - \frac{Ns_j^2\tau^2\rho}{\sigma^2(1-\rho)(1+\rho(Q-1))}\Lambda_j\mathbf{1}_Q\mathbf{1}_Q^T\right]^{-1} \\
&= \left[\left(\mathrm{I}_Q + \frac{Ns_j^2\tau^2}{\sigma^2(1-\rho)}\Lambda_j\right) - \frac{Ns_j^2\tau^2\rho}{\sigma^2(1-\rho)(1+\rho(Q-1))}\boldsymbol{\lambda}_j\mathbf{1}_Q^T\right]^{-1},
\end{aligned}$$

which is in the form of the Sherman-Morrison formula in (4), where $\boldsymbol{\lambda}_j = (\lambda_{j1}^2, \ldots, \lambda_{jQ}^2)^T$.

Here we have

$$\begin{aligned}
\mathrm{A} &= \mathrm{I}_Q + \frac{Ns_j^2\tau^2}{\sigma^2(1-\rho)}\Lambda_j \\
&= \mathrm{diag}\left(1 + \frac{Ns_j^2\tau^2}{\sigma^2(1-\rho)}\lambda_{j1}^2, \ldots, 1 + \frac{Ns_j^2\tau^2}{\sigma^2(1-\rho)}\lambda_{jQ}^2\right) \\
&= \mathrm{diag}\left(\frac{\sigma^2(1-\rho) + Ns_j^2\tau^2\lambda_{j1}^2}{\sigma^2(1-\rho)}, \ldots, \frac{\sigma^2(1-\rho) + Ns_j^2\tau^2\lambda_{jQ}^2}{\sigma^2(1-\rho)}\right), \\
\boldsymbol{u} &= -\frac{Ns_j^2\tau^2\rho}{\sigma^2(1-\rho)(1+\rho(Q-1))}\boldsymbol{\lambda}_j \text{ and} \\
\boldsymbol{v} &= \mathbf{1}_Q.
\end{aligned}$$

Thus, we have

$$\mathrm{A}^{-1} = \sigma^2(1-\rho)\mathrm{diag}\left\{\frac{1}{\sigma^2(1-\rho) + Ns_j^2\tau^2\lambda_{j1}^2}, \ldots, \frac{1}{\sigma^2(1-\rho) + Ns_j^2\tau^2\lambda_{jQ}^2}\right\}, \tag{5}$$

$$\begin{aligned}
\boldsymbol{u}\boldsymbol{v}^T\mathrm{A}^{-1} = &-\frac{Ns_j^2\tau^2\rho}{(1+\rho(Q-1))}\boldsymbol{\lambda}_j\mathbf{1}_Q^T \\
&\times \mathrm{diag}\left\{\frac{1}{\sigma^2(1-\rho) + Ns_j^2\tau^2\lambda_{j1}^2}, \ldots, \frac{1}{\sigma^2(1-\rho) + Ns_j^2\tau^2\lambda_{jQ}^2}\right\}
\end{aligned} \tag{6}$$

and

$$\begin{aligned}
&1+\boldsymbol{v}^T\mathrm{A}^{-1}\boldsymbol{u} \\
&= 1 - \frac{Ns_j^2\tau^2\rho}{(1+\rho(Q-1))}\mathbf{1}_Q^T\mathrm{diag}\left\{\frac{1}{\sigma^2(1-\rho) + Ns_j^2\tau^2\lambda_{j1}^2}, \ldots, \frac{1}{\sigma^2(1-\rho) + Ns_j^2\tau^2\lambda_{jQ}^2}\right\}\boldsymbol{\lambda}_j \\
&= 1 - \frac{Ns_j^2\tau^2\rho}{(1+\rho(Q-1))}\mathbf{1}_Q^T\left(\frac{\lambda_{j1}^2}{\sigma^2(1-\rho) + Ns_j^2\tau^2\lambda_{j1}^2}, \ldots, \frac{\lambda_{jQ}^2}{\sigma^2(1-\rho) + Ns_j^2\tau^2\lambda_{jQ}^2}\right)^T \\
&= 1 - \frac{Ns_j^2\tau^2\rho}{(1+\rho(Q-1))}\sum_{k=1}^{Q}\frac{\lambda_{jk}^2}{\sigma^2(1-\rho) + Ns_j^2\tau^2\lambda_{jk}^2} \\
&= \frac{(1+\rho(Q-1)) - Ns_j^2\tau^2\rho\sum_{k=1}^{Q}\frac{\lambda_{jk}^2}{\sigma^2(1-\rho)+Ns_j^2\tau^2\lambda_{jk}^2}}{(1+\rho(Q-1))}
\end{aligned} \tag{7}$$

Substituting in the values found in (5) to (7) into the Sherman-Morrison formula we have

$$\begin{aligned}
\mathcal{K}_j &= \sigma^2(1-\rho)\mathrm{diag}\left\{\frac{1}{\sigma^2(1-\rho)+Ns_j^2\tau^2\lambda_{j1}^2},\dots,\frac{1}{\sigma^2(1-\rho)+Ns_j^2\tau^2\lambda_{jQ}^2}\right\} \\
&\quad\times\left[\mathrm{I}_Q+\frac{Ns_j^2\tau^2\rho}{(1+\rho(Q-1))-Ns_j^2\tau^2\rho\sum_{k=1}^{Q}\frac{\lambda_{jk}^2}{\sigma^2(1-\rho)+Ns_j^2\tau^2\lambda_{jk}^2}}\right. \\
&\qquad\left.\times\,\mathrm{diag}\left\{\frac{1}{\sigma^2(1-\rho)+Ns_j^2\tau^2\lambda_{j1}^2},\dots,\frac{1}{\sigma^2(1-\rho)+Ns_j^2\tau^2\lambda_{jQ}^2}\right\}\right] \\
&= \mathrm{diag}\left\{\frac{1}{1+Ns_j^2\tau^2\lambda_{j1}^2(\sigma^2(1-\rho))^{-1}},\dots,\frac{1}{1+Ns_j^2\tau^2\lambda_{jQ}^2(\sigma^2(1-\rho))^{-1}}\right\} \\
&\quad\times\left[\mathrm{I}_Q+\frac{Ns_j^2\tau^2\rho}{1+\rho(Q-1)-Ns_j^2\tau^2\rho\sum_{k=1}^{Q}\frac{\lambda_{jk}^2}{\sigma^2(1-\rho)+Ns_j^2\tau^2\lambda_{jk}^2}}\boldsymbol{\lambda}_j\mathbf{1}_Q^T(\sigma^2(1-\rho))^{-1}\right. \\
&\qquad\left.\times\,\mathrm{diag}\left\{\frac{1}{1+Ns_j^2\tau^2\lambda_{j1}^2(\sigma^2(1-\rho))^{-1}},\dots,\frac{1}{1+Ns_j^2\tau^2\lambda_{jQ}^2(\sigma^2(1-\rho))^{-1}}\right\}\right] \\
&= \mathrm{diag}\left(\frac{1}{1+d_j^2\lambda_{j1}^2},\dots,\frac{1}{1+d_j^2\lambda_{jQ}^2}\right) \\
&\quad\times\left\{\mathrm{I}_Q+\frac{\rho d_j^2}{1-\rho+\rho\sum_{k=1}^{Q}\frac{1}{1+d_j^2\lambda_{jk}^2}}\boldsymbol{\lambda}_j\mathbf{1}_Q^T\mathrm{diag}\left(\frac{1}{1+d_j^2\lambda_{j1}^2},\dots,\frac{1}{1+d_j^2\lambda_{jQ}^2}\right)\right\},
\end{aligned}$$

where $d_j^2 = Ns_j^2\tau^2\left(\sigma^2(1-\rho)^{-1}\right)$ and $\boldsymbol{\lambda}_j = \left(\lambda_{j1}^2,\dots,\lambda_{jQ}^2\right)$. Therefore, the $(k,\ell)$-th element of $\mathcal{K}_j$ is

$$\mathcal{K}_{j,k\ell} = \begin{cases} \frac{1}{1+d_j^2\lambda_{jk}^2}\left\{1+\frac{\rho d_j^2\lambda_{jk}^2}{\left(1-\rho+\rho\sum_{m=1}^{Q}\frac{1}{1+d_j^2\lambda_{jm}^2}\right)(1+d_j^2\lambda_{jk}^2)}\right\}, & \text{if } k=\ell, \\ \frac{\rho d_j^2\lambda_{jk}^2}{\left(1-\rho+\rho\sum_{m=1}^{Q}\frac{1}{1+d_j^2\lambda_{jm}^2}\right)(1+d_j^2\lambda_{jk}^2)(1+d_j^2\lambda_{j\ell}^2)}, & \text{otherwise.} \end{cases}$$

We see that $\mathcal{K}_j$ is a rank-one update of a diagonal matrix. Thus, there is no closed form solution for the eigenvalues. As $\rho \to 0$, we obtain $\mathcal{K}_j$ when the error variance matrix is diagonal, shown in (12) of the main text (with $\sigma$ replaced with $\sigma_0$).

### 5.2.2 First order autoregressive case

Here we consider a variance matrix of a first order autoregressive time series of length $Q$, which is

$$\Sigma = \sigma^2\begin{pmatrix} 1 & \rho & \rho^2 & \cdots & \rho^{Q-1} \\ \rho & 1 & \rho & \cdots & \rho^{Q-2} \\ \vdots & \vdots & \vdots & \ddots & \vdots \\ \rho^{Q-1} & \rho^{Q-2} & \rho^{Q-3} & \cdots & 1 \end{pmatrix}$$

for which the stationarity condition is $|\rho| < 1$. The inverse is given by the symmetric, tridiagonal matrix

$$\Sigma^{-1} = \frac{1}{\sigma^2(1-\rho^2)} \begin{pmatrix} 1 & -\rho & 0 & \cdots & 0 & 0 & 0 \\ -\rho & 1+\rho^2 & -\rho & \cdots & 0 & 0 & 0 \\ \vdots & \vdots & \vdots & \ddots & \vdots & \vdots & \vdots \\ 0 & 0 & 0 & \cdots & -\rho & 1+\rho^2 & -\rho \\ 0 & 0 & 0 & \cdots & 0 & -\rho & 1 \end{pmatrix}.$$

Therefore, letting $d_j^2 = N s_j^2 \tau^2 \{\sigma^2(1-\rho^2)\}^{-1}$, we have

$$\mathcal{K}_j^{-1} = \begin{pmatrix} 1+d_j^2\lambda_{j1}^2 & -d_j^2\lambda_{j1}^2\rho & 0 & \cdots & 0 & 0 & 0 \\ -d_j^2\lambda_{j2}^2\rho & 1+d_j^2\lambda_{j2}^2(1+\rho^2) & -d_j^2\lambda_{j2}^2\rho & \cdots & 0 & 0 & 0 \\ \vdots & \vdots & \vdots & \ddots & \vdots & \vdots & \vdots \\ 0 & 0 & 0 & \cdots & -d_j^2\lambda_{j,Q-1}^2\rho & 1+d_j^2\lambda_{j,Q-1}^2(1+\rho^2) & -d_j^2\lambda_{j,Q-1}^2\rho \\ 0 & 0 & 0 & \cdots & 0 & -d_j^2\lambda_{jQ}^2\rho & 1+d_j^2\lambda_{jQ}^2 \end{pmatrix}$$

which is tridiagonal. As it is not Toeplitz, there is no closed-form solution for its eigenvalues. A closed-form for the inverse $\mathcal{K}_j$ is available but its hugely complicated structure prohibits further analytic manipulation.

## 5.3 Simulation study

As discussed in Section 5.2 of the main text, the density function for the joint distribution for $\mathcal{K}_j$ does not exist, except for the case when $\Sigma$ is diagonal. Here we explore the marginal and pairwise joint densities for elements of $\mathcal{K}_{j,kl}$ by simulation. We use the simplest non-diagonal special case of compound symmetry, where the diagonal elements of $\mathcal{K}_j$ will be identical and likewise for its off-diagonal elements (derived in Section 5.2.1).

Figure 24 shows kernel density estimates of the marginal densities for a diagonal and off-diagonal element when $Q \in \{2, 8, 14\}$, $\sigma = 1$ and the correlation parameter $\rho$ takes a range of values:

$$\begin{aligned} Q = 2: &\quad -0.50\ 0.00\ 0.50\ 0.95 \\ Q = 8: &\quad -0.12\ 0.00\ 0.50\ 0.95 \\ Q = 14: &\quad -0.07\ 0.00\ 0.50\ 0.95. \end{aligned}$$

The negative correlation is close to its smallest permissible value for each $Q$. In all cases, we take $N = s_j = 1$ and $\tau = 1$.

There are four distinct joint densities, between: a pair of diagonal elements; a pair of off-diagonal elements; a diagonal and off-diagonal element within the same row; and a diagonal and off-diagonal element in different rows. For each value of $Q$ and $\rho$, scatter plots of draws from the joint density are shown in Figure 4. For every combination of dimension $Q$ and correlation $\rho$, it is evident from the marginal and bivariate plots, that the diagonal elements of $\mathcal{K}_j$ retain the horseshoe shape from the univariate ($Q = 1$) case, with most of the density for the off-diagonal elements lying near the mode at 0. The horseshoe shape is evident in the marginal density plots of the diagonal elements. In the bivariate density plots of two diagonal elements, there are fewer points for values not near 0 or 1. Moreover, it seems that the off-diagonal elements are more likely to be close to zero, if the diagonal element in any particular row is close to one. For example, we can see in Figure 4 for all combinations of $Q$ and $\rho$ that when the diagonal element is close to 1, there is no density at values of the off-diagonal element greater than 0. When the diagonal element is close to 0, the off-diagonal element can take a value anywhere between 0 and $\rho$. This suggests that there is a high prior probability for values of $\mathcal{K}_j$ lying in the vicinity of diagonal matrices with ones and zeros on the diagonal.

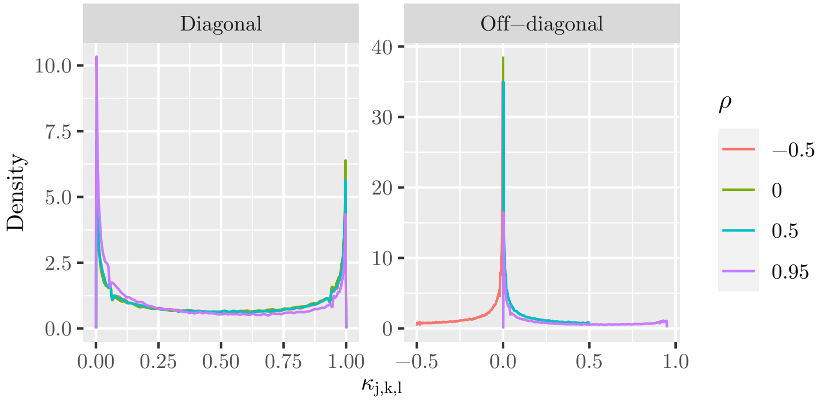


(a)

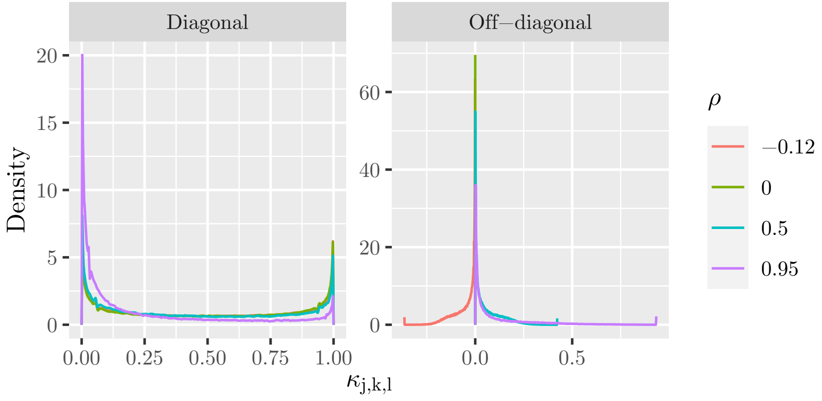


(b)

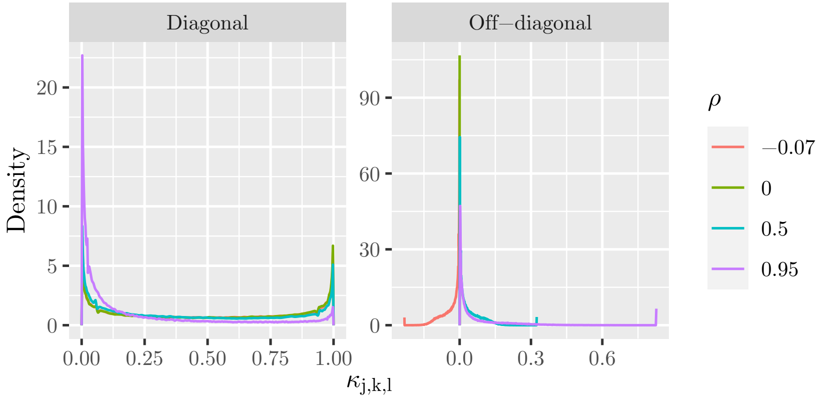


(c)

Figure 24: Conditional on the global shrinkage parameter $\tau$ and the error variance $\Sigma$, marginal densities of a diagonal and non-diagonal element of $\mathcal{K}_j$ when $\Sigma$ has compound symmetric structure and the dimension of the response vector is (a) $Q = 2$, (b) $Q = 8$ and (c) $Q = 14$. In each case, $\sigma = 1$, $N = s_j = 1$ and $\tau = 1$. A range of values for the correlation $\rho$ is considered.

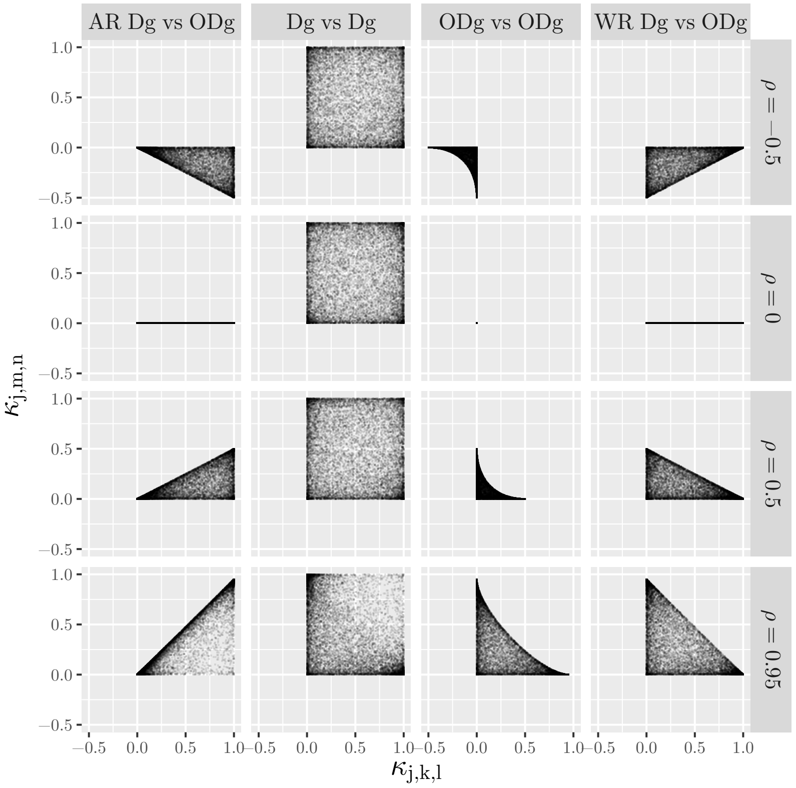
AR Dg vs ODg
Dg vs Dg
ODg vs ODg
WR Dg vs ODg
ρ = −0.5
ρ = 0
ρ = 0.5
ρ = 0.95
$\kappa_{j,m,n}$
$\kappa_{j,k,l}$

(a)

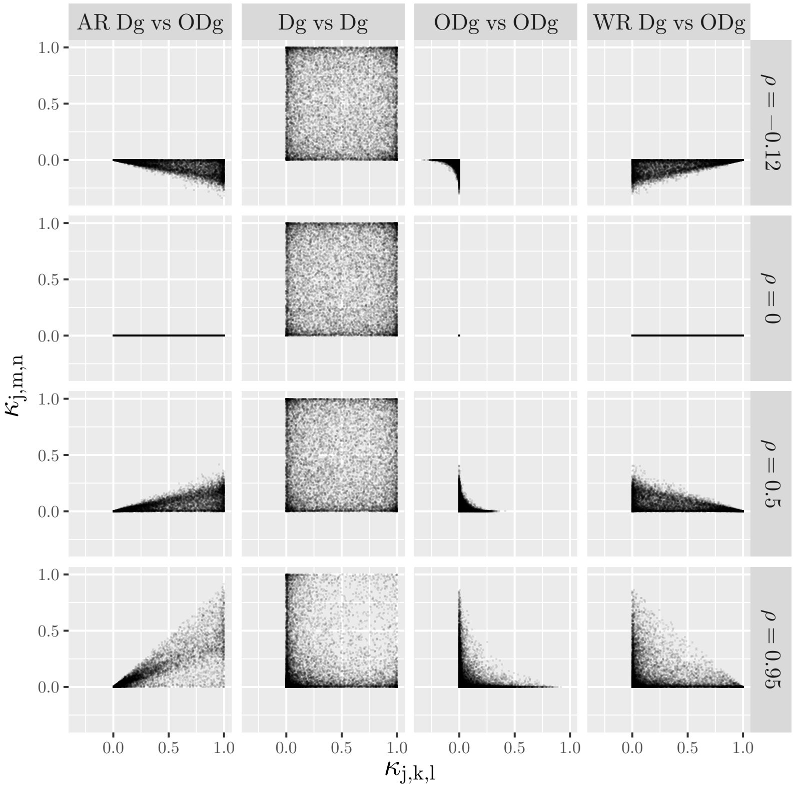
AR Dg vs ODg
Dg vs Dg
ODg vs ODg
WR Dg vs ODg
ρ = −0.12
ρ = 0
ρ = 0.5
ρ = 0.95
$\kappa_{j,m,n}$
$\kappa_{j,k,l}$

(b)

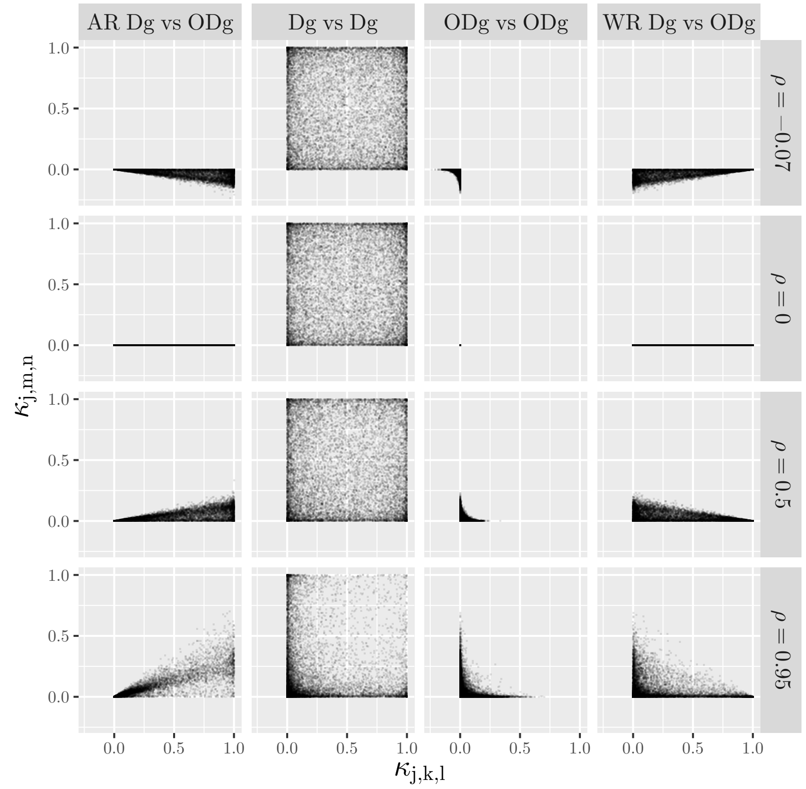


(c)

Figure 4: Conditional on the global shrinkage parameter $\tau$ and error variance $\Sigma$, pairwise bivariate densities between a pair of diagonal elements of $\mathcal{K}_j$ (Dg vs Dg); a pair of off-diagonal elements (ODg vs ODg); a diagonal and off-diagonal element within the same row (WR Dg vs ODg); and a diagonal and off-diagonal element in different rows (AR Dg vs ODg) when $\Sigma$ has compound symmetric structure and the dimension of the response vector is (a) $Q = 2$, (b) $Q = 8$ and (c) $Q = 14$. In each case, $\sigma = 1$, $N = s_j = 1$ and $\tau = 1$. A range of values for the common correlation $\rho$ is considered.

# 6 Choices of prior for unstructured $\Sigma$

For unstructured $\Sigma$, there are many options for the conditional distribution for $\Sigma|\sigma$. One simple possibility is the inverse Wishart distribution, that is

$$\Sigma|\sigma \sim \mathcal{W}^{-1}\left\{\sigma^2(\nu - K - 1)\mathrm{I}_K, \nu\right\},$$

where $\nu > K + 3$ to ensure that the distribution has finite variance. As it is a conjugate prior, the inverse Wishart is computationally convenient. However, it is very restrictive and inflexible (Daniels and Pourahmadi, 2002). The main issue is that a single hyperparameter $\nu$ is used to control the distributional properties of all elements in $\Sigma$.

A better option for an unconstrained $\Sigma$ would be to decompose $\Sigma = \mathrm{DRD}$ where $\mathrm{D} = \mathrm{diag}\left(\sigma_1, ..., \sigma_K\right)$ is a diagonal matrix of standard deviations $\sigma_i = \sqrt{\Sigma_{ii}}$ and $\mathrm{R} = (R_{ij})$ is a matrix of correlations $R_{ij} = \Sigma_{ij}/\left(\sigma_i\sigma_j\right)$. Then we could assign the prior

$$\pi\left(\Sigma|\sigma\right) = \pi(\mathrm{R})\prod_{i=1}^{K}\pi\left(\sigma_i^2|\sigma\right),$$

giving the $\sigma_i$ some distribution on $\mathbb{R}^+$ with $\mathrm{E}\left(\sigma_i^2|\sigma\right) = \sigma^2$ and R some distribution over the space of $K \times K$ correlation matrices such that $\mathrm{E}\left(R_{ij}\right) = 0$, for all $i \neq j$. For instance, we could

have

$$\sigma_i | \sigma \sim \text{LN}\left\{\log(a), \log\left(\sigma/a\right)\right\},$$

where $a$ is the median of $\sigma_i$ and assign to R the (proper) jointly uniform distribution, $\pi\left(\text{R}\right) \propto 1$. In other words, we could assign equal prior density to all possible $K \times K$ correlation matrices.

Instead of specifying a prior for the covariance matrix, we could instead specify a prior for the precision matrix $\Sigma^{-1}$. Similarly, when $\Sigma^{-1}$ is unstructured, there is a variety of options for the conditional distribution for $\Sigma^{-1}|\sigma$. A reasonable approach would be to reparameterise $\Sigma^{-1}$ in terms of its square-root free Cholesky decomposition (Daniels and Pourahmadi, 2002) $\Sigma^{-1} = \text{T}^T\text{D}^{-1}\text{T}$, where $\text{D} = \text{diag}\left(\sigma_1, \ldots, \sigma_K\right)$ and T is a lower triangular matrix with 1s on the diagonal and its $(i, j)$-th entry is $-\phi_{i,j}$ for $i > j$. This gives a new set of real valued parameters that are unconstrained, unlike the original covariance matrix, which must be symmetric and positive definite. However, for the parameters to be interpretable, the data must have some order. Our clustered data have a circular time-ordering, with the OTUs in neighbouring bins (or bins 12 and 1), typically peaking in abundance in neighbouring months. Therefore, the square-root free Cholesky decomposition might have been sensible for our data if we had opted to allow $\Sigma$ to be unconstrained. Instead, we choose a more parsimonious option by using a symmetric, circulant, tridiagonal precision matrix (Section 4.1 of the main text).

# 7 Stan code

Here we present our Stan code for our model.

Listing 1: Code for the VAR(1) model used for the WWTP data.

```
// Stan code for VAR(1) model in Hannaford et al. 2021
functions {

}

data {
  int<lower = 1> K;                              // No. of bins/columns in data
  int<lower = 1> N;                              // No. of time points/rows in data
  int<lower = 1> N_miss;                         // No. time points missing from data
  matrix[N-N_miss,K] y_obs;                      // Observed data
  int<lower = 1, upper = N> which_y_miss[N_miss];   // Indices of missing time points
  int<lower = 1, upper = N> which_y_obs[N-N_miss]; // Indices of observed time points
  row_vector[N] intercept_X;                       // Intercept term for design matrix
  int<lower=1> L;                                  // Number of CE covariates + 1 (for intercept)
  int<lower=0> N_Nitrate_obs;                    // Number of observed Nitrate values
  int<lower=0> N_COD_obs;                        // Number of observed COD values
  int<lower=0> N_Ammonia_obs;                    // Number of observed Ammonia values
  int<lower=0> N_pH_obs;                         // Number of observed pH values
  int<lower=0> N_Phosphate_obs;                  // Number of observed phosphate values


  row_vector[N_Nitrate_obs] Nitrate_obs; //  Observed values for Nitrate
  row_vector[N_COD_obs] COD_obs;         //  Observed values for COD
  row_vector[N_Ammonia_obs] Ammonia_obs; //  Observed values for Ammonia
  row_vector[N_pH_obs] pH_obs;           //  Observed values for pH
  row_vector[N_Phosphate_obs] Phosphate_obs; // Observed values for phosphate


  int <lower = 1, upper = N> which_Nitrate_miss[N-N_Nitrate_obs];
  //  Indices of missing values for Nitrate
  int <lower = 1, upper = N> which_COD_miss[N-N_COD_obs];
  //  Indices of missing values for COD
  int <lower = 1, upper = N> which_Ammonia_miss[N-N_Ammonia_obs];
  //  Indices of missing values for Ammonia
  int <lower = 1, upper = N> which_pH_miss[N-N_pH_obs];
  //  Indices of missing values for pH
  int <lower = 1, upper = N> which_Phosphate_miss[N-N_Phosphate_obs];
  //  Indices of missing values for Phosphate
  int <lower = 1, upper = N> which_Nitrate_obs[N_Nitrate_obs];
  //  Indices of observed values for Nitrate
  int <lower = 1, upper = N> which_COD_obs[N_COD_obs];
  //  Indices of observed values for COD
    int <lower = 1, upper = N> which_Ammonia_obs[N_Ammonia_obs];
  //  Indices of observed values for Ammonia
  int <lower = 1, upper = N> which_pH_obs[N_pH_obs];
  //  Indices of observed values for pH
  int <lower = 1, upper = N> which_Phosphate_obs[N_Phosphate_obs];
  //  Indices of observed values for Phosphate

  int<lower=1> Nh;                         //  Number of harmonics for mu
  real<lower = 0> global_scale;            //  tau_0 (scale for global shrinkage)
  real<lower=0> slab_scale;                //  Slab scale for the regularised horseshoe
  real<lower=0> slab_df;                   //  Slab DOF for the regularised horseshoe
  real m_beta;                             //  Prior mean for beta
```

```
  real<lower=0> v_beta;                 //  Prior variance for beta
  real m_gamma;                         //  Prior mean for gamma
  real<lower=0> v_gamma;                //  Prior variance for gamma
  real<lower=1> nu_local;               //  Degrees of freedom for half-t prior for tau
  real<lower=1> nu_global;              //  Degrees of freedom for half-t prior for lambdas
                                        //  nu_global = nu_local = 1 gives half-Cauchy.
  real<lower=0> s_sigma;                //  Prior sd for lognormal for sigma
  real<lower=0> c_error;                //  Prior coefficient of variation for omega_1, omega_2
  real a_alpha;                         //  Prior mean for means_B
  real<lower=0> b_alpha;                //  Prior sd for means_B
  real<lower=2> c_alpha;                //  Prior shape for sigma_sq_B
  real<lower=0> d_alpha;                //  Prior scale for sigma_sq_B
  real<lower=0> alpha_phi;              //  Shape 1 for beta prior for phi
  real<lower=0> beta_phi;               //  Shape 2 for beta prior for phi
  real<lower = (L+2)> nu;               //  Prior degrees of freedom - inv. Wishart for Sigma_X
  cov_matrix[(L-1)] S_X;                //  Prior scale matrix - inv. Wishart for Sigma_X
}

transformed data {
  // sin. and cos. values for mu
  matrix[Nh,N] sin_mat;
  matrix[Nh,N] cos_mat;
  real pi_const = (2*pi())/52;
  for(j in 1:Nh) {
    for(t in 1:N) {
      sin_mat[j,t] = pi_const*j*t;
      cos_mat[j,t] = sin_mat[j,t];
    }
  }

  sin_mat = sin(sin_mat);
  cos_mat = cos(cos_mat);

}

parameters {
  matrix[K,K] z;
  matrix[Nh,K] beta;              // Beta params (sin. fourier coefficient) for mu
  matrix[Nh,K] gamma;           // Gamma params (cos. fourier coefficient) for mu
  matrix[N_miss, K] y_miss;     // Missing y values
  real<lower=0> omega_0;
  real<lower=0> omega_1;
  real<lower=0> caux;
  real<lower=0> aux1_global;
  real<lower=0> aux2_global;
  matrix<lower=0>[K,K] aux1_local;
  matrix<lower=0>[K,K] aux2_local;
  real<lower=0> sigma;
  vector[L] means_B;                                      // Prior means for alpha
  real<lower=0> sigma_sq_B[L];                            // Prior variance parameters for alphas
  matrix[L,K] B_tilde;                                    // Used to get regression coefficients
  row_vector[N-N_Nitrate_obs] Nitrate_miss;               // Missing value for Nitrate
  row_vector[N-N_COD_obs] COD_miss;                       // Missing values for COD
  row_vector[N-N_Ammonia_obs] Ammonia_miss;               // Missing values for Ammonia
  row_vector[N-N_pH_obs] pH_miss;                         // Missing values for pH
  row_vector[N-N_Phosphate_obs] Phosphate_miss;           // Missing values for Phosphate.
  vector<lower=0, upper=1>[L-1] phi;                      // Phi for imputing missing values (AR coefficient)
  cov_matrix[L-1] Sigma_X;                                // Sigma_X for imputing missing values
}

transformed parameters {
  real<lower=0> tau;                    //  Global shrinkage parameter
  matrix<lower=0>[K,K] lambda;          //  Local shrinkage parameter
  matrix<lower=0>[K,K] lambda_tilde;    // 'Truncated' local shrinkage parameter
  real<lower=0> c;
  matrix[K,K] A;                        //  Coefficient matrix
  real<lower=0> sigma_0;
  real omega;
  matrix[K,K] precision_matrix;         // Precision matrix of errors
  matrix[N,K] alpha;                    // Alpha (intercept for mu)
  matrix[N,K] mu;                       // Time varying mean
  matrix[L,K] B;                        // Regression coefficients for alpha
  matrix[L,N] X;                        // Design matrix with missing values imputed
  matrix[N,K] y;                        // Data constructed from y_obs and y_miss

  y[which_y_obs,] = y_obs;
  y[which_y_miss,] = y_miss;

  X[2,which_Nitrate_miss] = Nitrate_miss;
  X[2,which_Nitrate_obs] = Nitrate_obs;
  X[3,which_COD_miss] = COD_miss;
  X[3,which_COD_obs] = COD_obs;
  X[4,which_Ammonia_miss] = Ammonia_miss;
  X[4,which_Ammonia_obs] = Ammonia_obs;
  X[5,which_pH_miss] = pH_miss;
  X[5,which_pH_obs] = pH_obs;
  X[6,which_Phosphate_miss] = Phosphate_miss;
  X[6,which_Phosphate_obs] = Phosphate_obs;
  X[1,] = intercept_X;

  // Error precision matrix
  sigma_0 = (omega_0+omega_1)/sqrt(2);           // sigma_0 main diagonal of precision
  omega = (omega_0-omega_1)/(2*sqrt(2));         // omega super-, sub-diagonals of precision.
                                                 // top right, bottom left corners

  precision_matrix = rep_matrix(0.0, K,K);
  precision_matrix[1,K] = omega;
  precision_matrix[K,1] = omega;
  precision_matrix[K,K] = sigma_0;
```

```
  for(j in 1:(K-1)) {
    precision_matrix[j,j] = sigma_0;
    precision_matrix[j,(j+1)] = omega;
    precision_matrix[(j+1),j] = omega;
  }

  // mu
  for(l in 1:L) {
    B[l,] = B_tilde[l,] * sigma_sq_B[l];
  }
  for(i in 1:N) {
    alpha[i,] = (B'*X[,i])';
                mu[i,] =  alpha[i,];
                for(j in 1:Nh) {
                  mu[i,] += (beta[j,]*sin_mat[j,i] + gamma[j,]*cos_mat[j,i]);
                }
  }

  // A
  c = slab_scale * sqrt(caux);
  tau = aux1_global * sqrt(aux2_global) * global_scale * sigma;
  for(i in 1:K) {
    lambda[i,] = aux1_local[i,] .* sqrt(aux2_local[i,]);
    lambda_tilde[i,] = sqrt(c^2*square(lambda[i,]) ./ (c^2 +tau^2*square(lambda[i,])));
    A[i,] =  z[i,] .* lambda_tilde[i,]*tau;
  }
}


model {
  real c_inv = 1/c_error^2;
  vector[L-1] mean_X;

  // Prior for error precision matrix (reparameterisation)
  sigma ~ lognormal(0, s_sigma);
  omega_0 ~ gamma(c_inv, sqrt(2)*sigma^2*c_inv);
  omega_1 ~ gamma(c_inv, sqrt(2)*sigma^2*c_inv);

  // CE covariates
  phi ~ beta(alpha_phi, beta_phi);
  Sigma_X ~ inv_wishart(nu, S_X);
  for(i in 2:N) {
    mean_X = phi .* X[2:L,i-1];
    X[2:L,i] ~multi_normal(mean_X,Sigma_X);
  }

  // Prior for B (alpha)
  means_B ~ normal(a_alpha, b_alpha);
  sigma_sq_B ~ inv_gamma(c_alpha, d_alpha);
  for(l in 1:L) {
    B_tilde[l,] ~ normal(means_B[l],1);
  }

  // Prior for beta and gamma
  for(j in 1:Nh) {
    beta[j,] ~ normal(m_beta, sqrt(v_beta));
    gamma[j,] ~ normal(m_gamma, sqrt(v_gamma));
  }

  // Half t-priors for lambdas and tau, and inverse-gamma for c^2
  // Half cauchy if nu_local = nu_global = 1
  for(i in 1:K) {
    z[i,] ~ normal(0,1);
    aux1_local[i,]~normal(0,1);
    aux2_local[i,]~inv_gamma(0.5*nu_local, 0.5*nu_local);
  }
  aux1_global ~ normal(0,1);
  aux2_global ~ inv_gamma(0.5*nu_global, 0.5*nu_global);

  caux ~ inv_gamma(0.5*slab_df, 0.5*slab_df);

  // Mu and Likelihood
  for(i in 2:N) {
    y[i,] ~ multi_normal_prec(mu[i,]'+A*(y[(i-1),]'-mu[i-1,]'), precision_matrix);
  }

}
```

# 8 Application

## 8.1 Posterior means and CIs of parameters

The posterior means and 95% credible intervals (CIs) for the regression coefficients of nitrate and phosphate are shown in Figure 5. All of the CIs overlap zero, which may suggest that neither nitrate or phosphate have a linear relationship with any of the bins. Nevertheless, there is some evidence of "winter blooming" bins having a positive relationship with phosphate and "summer blooming" bins having a negative relationship with phosphate. However, this could be an artefact of how the OTUs were clustered.

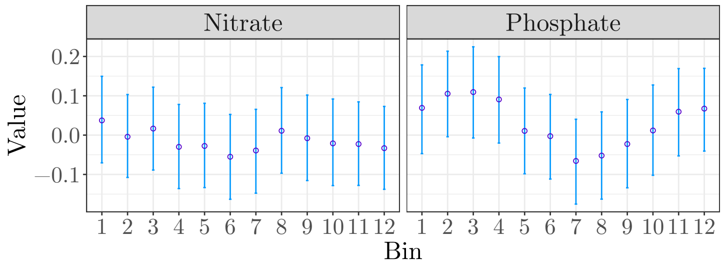


Figure 5: Posterior means (∘) and 95% credible intervals (—) for nitrate and phosphate (AS tank).

The posterior means and 95% CIs for the harmonic regression coefficients $\boldsymbol{\beta}_j$ and $\boldsymbol{\gamma}_j$ are shown in Figures 6 and 7, respectively. In Figure 8, the posterior means and 95% CIs are shown for the time varying mean $\boldsymbol{\mu}_t$. They are plotted over the scaled log counts of each bin. All these plots are discussed in Section 7.1.2 of the main text.

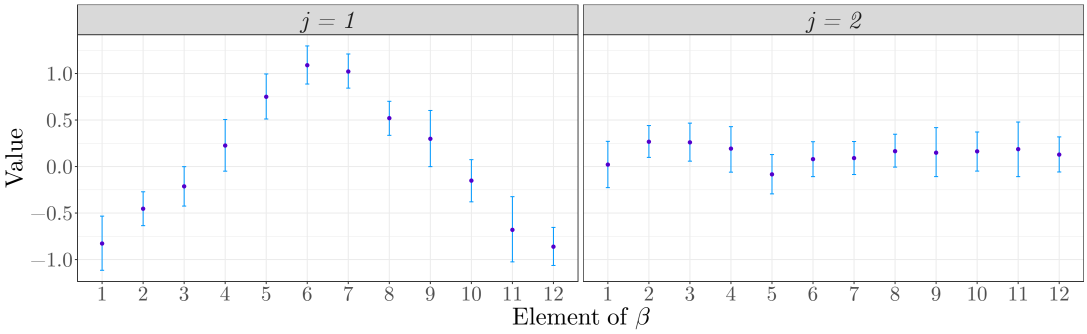


Figure 6: Posterior means (∘) and 95% credible intervals (—)of the harmonic regression coefficients $\boldsymbol{\beta}_j$.

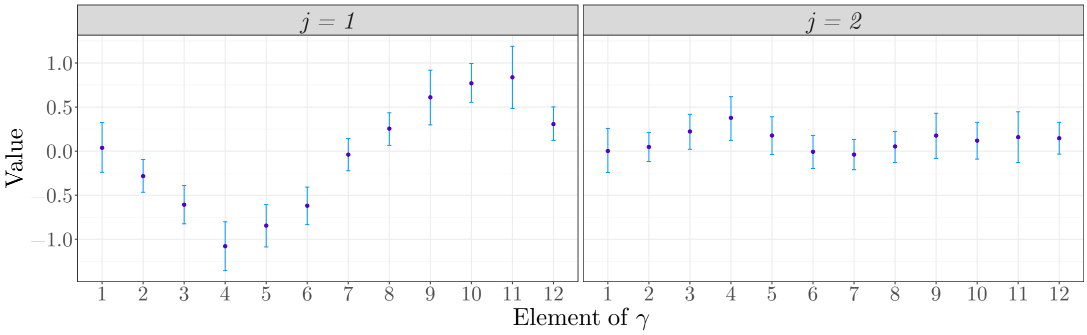


Figure 7: Posterior means (∘) and 95% credible intervals (—) of the harmonic regression coefficients $\boldsymbol{\gamma}_j$.

Figure 9 shows the posterior means and 95% CIs of the lag-$k$ correlations $\rho_k$ and is discussed in Section 7.3 of the main text.

## 8.2 Most abundant OTUs in each bin

The most abundant OTUs in each bin are listed in Table 5. This information is used in the Section 7 of the main text to aid biological interpretation of the results.

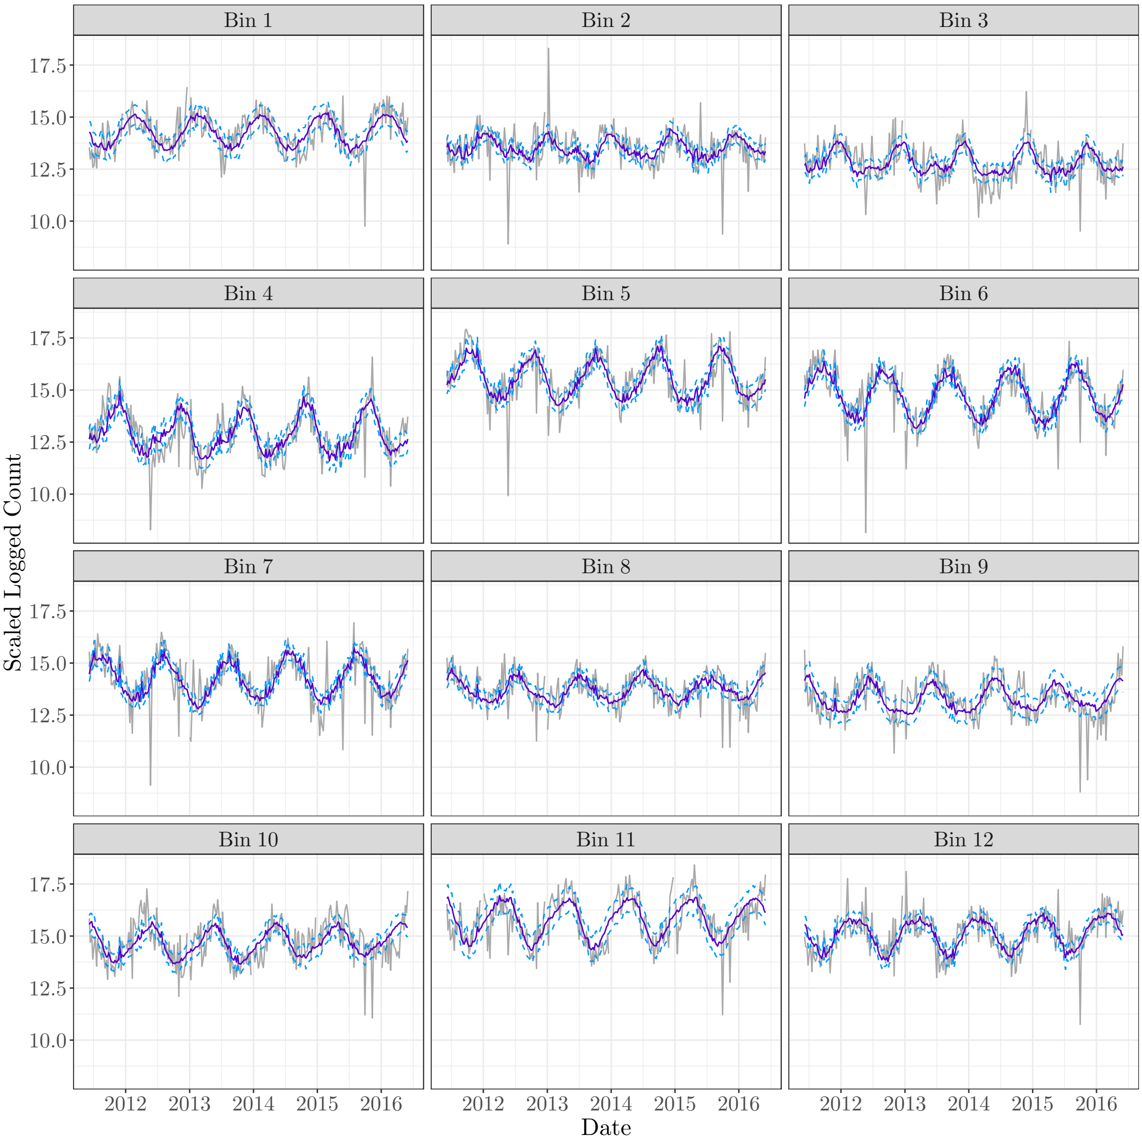


Figure 8: Posterior means (—) and 95% credible intervals (- - -) for the time varying means with scaled log counts (—) for each bin.

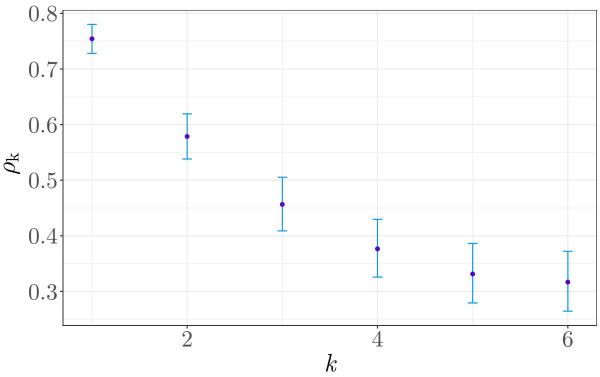


Figure 9: Posterior means (∘) and 95% credible intervals (—) of the lag-$k$ correlations $\rho_k$ for $k = 1, \ldots, 6$.

| Bin | Genera |
|---|---|
| 1 | *Tabrizicola*, *Rhodobacter*, *Methylorosula*, *Ruminococcus* 2, *Fusicatenibacter*, *Albidiferax* |
| 2 | Unknown (Family: *Rhodobacteraceae*, 2), *Haematobacter*, *Polymorphobacter*, *Thermomonas*, *Novosphingobium* |
| 3 | *Amaricoccus*, Unknown (Family: *Microbacteriaceae*), *Paracoccus* (2), CL500-29 marine group, *Ca. Microthrix* |
| 4 | *Terrimonas*, *Ca. Microthrix*, *Zymomonas*, *Acinetobacter*, *Phenylobacterium*, *Nitrospira* |
| 5 | *Zoogloea*, *Acidovorax*, *Ca. Microthrix*, *Afipia*, *Simplicispira*, *Iamia* |
| 6 | Unknown (Family: *Alcaligenaceae*), Unknown (Family: MN67), *Dokdonella*, *Dechloromonas*, *Piscinibacter*, *Rhizobium* |
| 7 | *Leptothrix*, *Dechloromonas*, Unknown (Family: *Cytophagaceae*, *Hirschia*, Unknown (Family: *Saprospiraceae*), *Iamia* |
| 8 | *Romboutsia*, Unknown (Family: *Comamonadaceae*), *Devosia*, *Lautropia*, Unknown (Family: Unknown), *Lacibacter* |
| 9 | *Defluviimonas*, *Intestinibacter*, *Nitrosomonas*, *Hyphomicrobium*, *Ferruginibacter* (2) |
| 10 | Unknown (Family: Gsoil-1167), *Ca. Microthrix*, *Rhizobacter*, *Defluviimonas*, Unknown (Family: *Rhodobacteraceae*), *Ca. Nitrotoga* |
| 11 | Unknown (Family: *Saprospiraceae*, 2), *Defluviimonas*, *Terrimonas* (2), *Rhodoferax* |
| 12 | *Trichococcus*, *Rhodobacter* (3), *Ornithinibacter*, *Subdoligranulum* |

Table 5: Genera of the top six OTUs in each bin based on median relative abundance.

## References


Daniels, M. J., Pourahmadi, M., 2002. Bayesian analysis of covariance matrices and dynamic models for longitudinal data. Biometrika 89 (3), 553–566.

Hoffman, M. D., Gelman, A., 2014. The No-U-Turn Sampler: Adaptively setting path lengths in Hamiltonian Monte Carlo. Journal of Machine Learning Research 15, 1593–1623.

Kuo, L., Mallick, B., 1998. Variable selection for regression models. Sankhyā: The Indian Journal of Statistics, Series B (1960-2002) 60 (1), 65–81.

Lei, G., Boys, R. J., Gillespie, C. S., Greenall, A., Wilkinson, D. J., 2011. Bayesian inference for sparse VAR (1) models, with application to time course microarray data. Journal of Biometrics & Biostatistics 2 (5).

O'Hara, R., Sillanpää, M., 2009. A review of Bayesian variable selection methods: What, how and which. Bayesian Analysis 4 (1), 85–118.

Stan Development Team, 2020. Stan modeling language users guide and reference manual, version 2.25.
URL `https://mc-stan.org`
